# Supplementary material for: Observation of dislocation bound states and skin effects in non-Hermitian Chern insulators
Source: arXiv:2504.02824 ancillary file (2026-01-29)
Supplement: Supplementary file 1 [file SuppMat_APS.pdf]

# Supplementary Materials

## “Observation of non-Hermitian dislocation bound states and dislocation skin effects”

Jia-Xin Zhong<sup>1</sup>, Bitan Roy<sup>\*2</sup>, and Yun Jing<sup>†1</sup>

<sup>1</sup>Graduate Program in Acoustics, The Pennsylvania State University, University Park, PA 16802, USA

<sup>2</sup>Department of Physics, Lehigh University, Bethlehem, Pennsylvania 18015, USA

### Contents

|                                                                                                |           |
|------------------------------------------------------------------------------------------------|-----------|
| <b>S1 Phase diagram of NH Chern insulators</b>                                                 | <b>2</b>  |
| <b>S2 Experimental details</b>                                                                 | <b>4</b>  |
| S2.1 Overall structure and measurement process                                                 | 4         |
| S2.2 Acoustic cavities and tuning of onsite potentials                                         | 5         |
| S2.3 Tuning of hoppings                                                                        | 6         |
| S2.4 The coupled-model theory for the unidirectional coupling of two coupled acoustic cavities | 7         |
| <b>S3 Extended experimental results</b>                                                        | <b>9</b>  |
| <b>References</b>                                                                              | <b>38</b> |

---

<sup>\*</sup>bitan.roy@lehigh.edu

<sup>†</sup>yqj5201@psu.edu

## S1 Phase diagram of NH Chern insulators

In this section of the Supplemental Material, we discuss the phase diagram of the Bloch Hamiltonian for 2D non-Hermitian (NH) Chern insulator given by

$$H_{\text{NH}}(\mathbf{k}) = H_{\text{H}}(\mathbf{k}) + i\boldsymbol{\sigma} \cdot \mathbf{h} = \boldsymbol{\sigma} \cdot [\mathbf{d}(\mathbf{k}) + i\mathbf{h}] \equiv \boldsymbol{\sigma} \cdot \mathbf{d}_{\text{NH}}(\mathbf{k}), \quad (\text{S1})$$

where

$$\mathbf{d}(\mathbf{k}) = (t_0 \sin k_x + ih_x, t_0 \sin k_y + ih_y, t_0 [\cos k_x + \cos k_y] - m_0 + ih_z). \quad (\text{S2})$$

The phase diagram of this model is determined from the NH Chern number given by

$$C = \text{Re} \int_{\text{BZ}} \frac{d^2 \mathbf{k}}{4\pi} [\partial_x \hat{\mathbf{d}}_{\text{NH}}(\mathbf{k}) \times \partial_y \hat{\mathbf{d}}_{\text{NH}}(\mathbf{k})] \cdot \hat{\mathbf{d}}_{\text{NH}}(\mathbf{k}), \quad (\text{S3})$$

where  $\partial_j \equiv \partial_{k_j}$ ,  $\mathbf{d}_{\text{NH}}(\mathbf{k}) = \mathbf{d}(\mathbf{k}) + i\mathbf{h}$ , and  $\hat{\mathbf{d}}_{\text{NH}}(\mathbf{k}) = \mathbf{d}_{\text{NH}}(\mathbf{k}) / \sqrt{\mathbf{d}_{\text{NH}}^2(\mathbf{k})}$ . For  $\mathbf{h} = 0$ , we recover the standard definition of the Chern number. The integration is performed within the first Brillouin zone.

The phase diagram of  $H_{\text{NH}}(\mathbf{k})$ , obtained in terms of  $C$  is shown in Fig. S1. For  $h_x$  or  $h_y$ , the red shaded region in Fig. S1(a) where  $C = -1$  is determined by

$$\begin{cases} |h_x| < |m_0 + 2|, & -2 \leq m_0/t_0 \leq -1 \\ |h_x| < |m_0|, & -1 \leq m_0/t_0 \leq 0. \end{cases} \quad (\text{S4})$$

On the same phase diagram the blue shaded region where  $C = 1$  is determined by

$$\begin{cases} |h_x| < |m_0 - 2|, & 1 \leq m_0/t_0 \leq 2 \\ |h_x| < |m_0|, & 0 \leq m_0/t_0 \leq 1. \end{cases} \quad (\text{S5})$$

On the other hand, for  $h_z$ , the red shaded region in Fig. S1(b) where  $C = -1$  is determined by

$$|h_z| < \sqrt{2|m_0| - m_0^2}, \quad -2 \leq m_0/t_0 \leq 0. \quad (\text{S6})$$

Whereas the blue shaded region where  $C = 1$  is determined by

$$|h_z| < \sqrt{2|m_0| - m_0^2}, \quad 0 \leq m_0/t_0 \leq 2. \quad (\text{S7})$$

Outside these parameter regimes, shown by the white shaded regions in Fig. S1, the NH Chern number is trivial. Respectively, in the red and blue shaded regions the inversion of the NH and Hermitian (when  $\mathbf{h} = 0$ ) bands occur near the M and  $\Gamma$  points of the Brillouin zone.

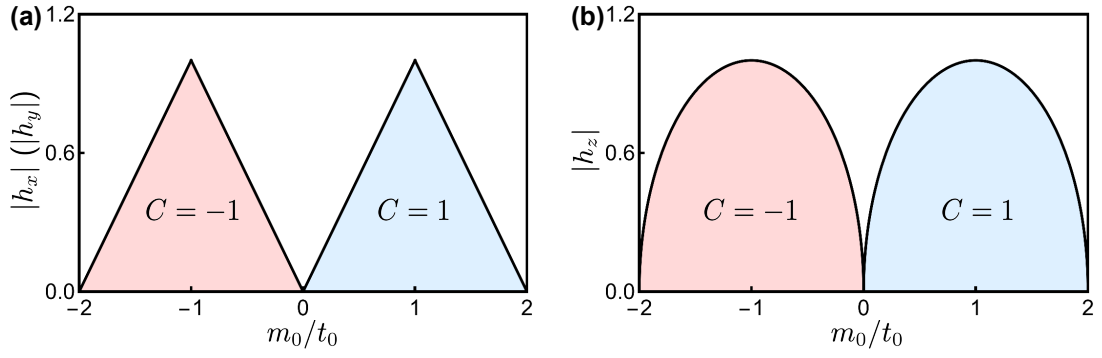

**Figure S1:** Phase diagram of NH Chern insulators with NH perturbations for (a)  $h_x$  (or  $h_y$ ) and (b)  $h_z$ . The eigenenergies are line-gapped only in the red and blue shaded regions, where the NH Chern number is  $C = -1$  and  $C = 1$ , respectively. The system supports topologically protected dislocation states only in the red shaded regions.

## S2 Experimental details

This section of the Supplemental Material is devoted to discuss various key details related to the implementation of NH model on acoustic lattice and measurement protocols.

### S2.1 Overall structure and measurement process

Figure S2 shows a photograph of our experimental setup. The system consists of 56 3D-printed acoustic cavities, each representing a site in the NH lattice. A custom-designed digital controller is employed to precisely tune the onsite potentials of the acoustic cavities and the hoppings between them, as detailed in Secs. S2.2 and S2.3, respectively. The tuning of onsite potentials and hoppings is implemented using active components, specifically microphone-loudspeaker (detector-source) pairs. The hopping implementations are independent of spatial distances between sites, enabling flexible implementation of various boundary conditions and lattice geometries with ease.

The custom-made digital controller comprises three components: the core board, the motherboard, and the input/output (IO) board. The core board houses a field-programmable gate array (FPGA, XC7K325T, Xilinx) and a digital signal processor (DSP, TMS320C6678, Texas

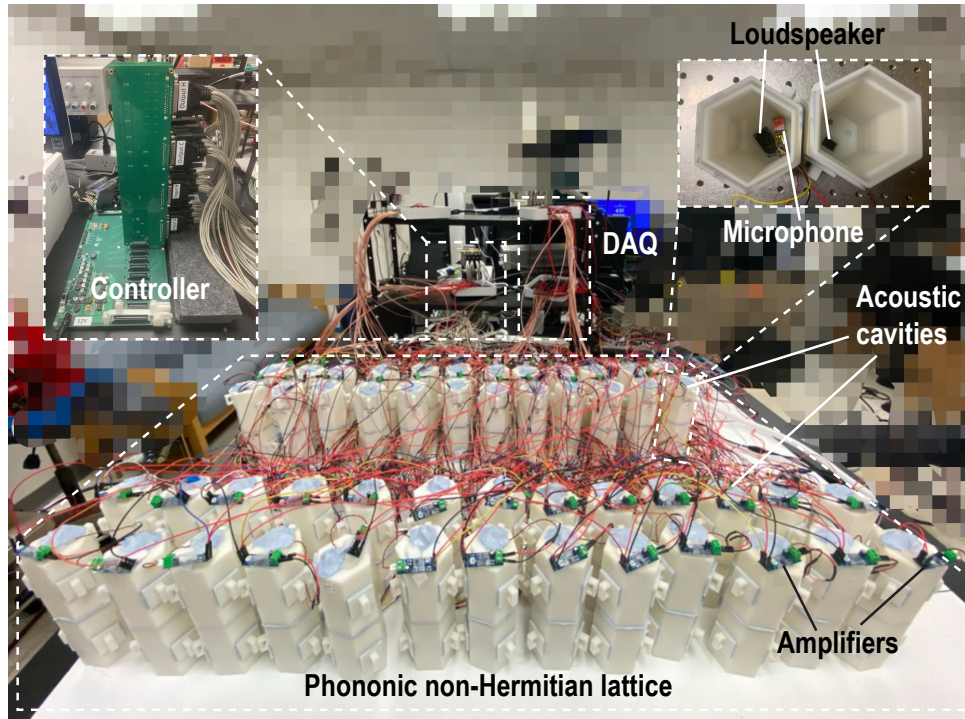

**Figure S2: Photo of the experimental setup.** The phononic non-Hermitian lattice consists of 56 acoustic cavities. Onsite potential and hoppings are implemented using microphone-loudspeaker pair. The magnitude and phase of hoppings are tuned using a real-time digital controller. A data acquisition (DAQ) system is programmed to measure the Green's function for all possible combinations of source-detector positions across the entire lattice.

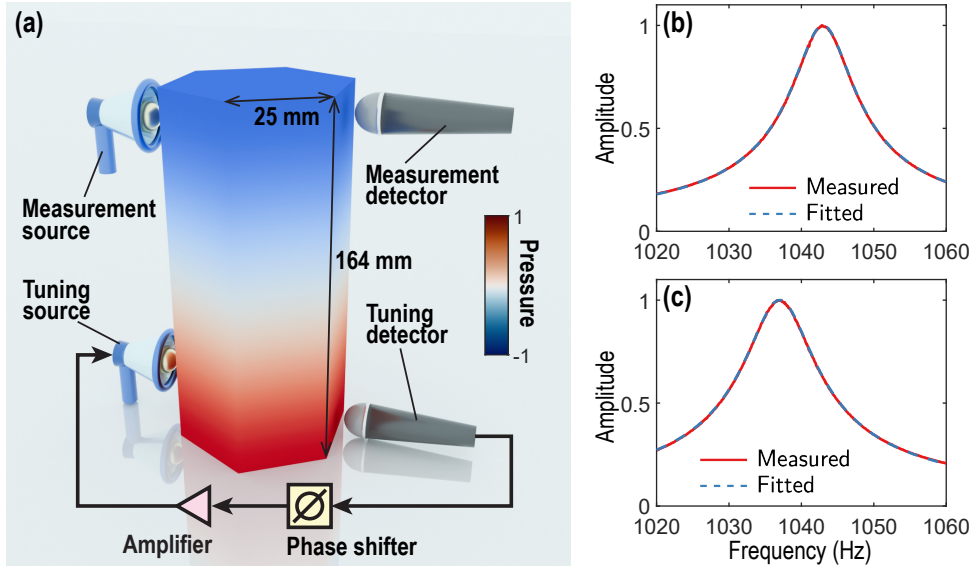

**Figure S3: Tuning onsite potential (resonant frequency) of acoustic cavities.** (a) Schematic illustration of the tuning process. The air column is designed as a hexagonal prism with a height of 164 mm and a side length of 25 mm. (b–c) Measured and fitted magnitude responses for two typical configurations that emulate the sublattices: (b) sublattice ‘A’ and (c) sublattice ‘B’ within a unit cell. In (b), the target onsite potential is  $\omega_0 - m_0 + i h_z = 1043 \text{ Hz} - 4.2i \text{ Hz}$ , and the value obtained from fitting experimental data is  $1042.98 \text{ Hz} - 4.21i \text{ Hz}$ . In (c), the target onsite potential is  $\omega_0 + m_0 - i h_z = 1037 \text{ Hz} - 4.8i \text{ Hz}$ , with the fitted value being  $1037.00 \text{ Hz} - 4.81i \text{ Hz}$ . Other parameters are  $\omega_0 = 1040 \text{ Hz} - 4.5i \text{ Hz}$ ,  $m_0 = -3 \text{ Hz}$ , and  $h_z = 0.3 \text{ Hz}$ .

Instruments), which enable real-time signal processing. During experiments, the system operates at a sampling frequency of 12.8 kHz. The motherboard supplies power and facilitates communication between the core and IO boards. The IO board handles analog signal acquisition and output, interfacing with microphones and loudspeakers, respectively. Each IO board supports 16 channels for both analog inputs and outputs. The input channels utilize analog-to-digital converters (ADCs, ADC7606B, ADI), and the output channels employ digital-to-analog converters (DACs, DAC8568, Texas Instruments).

To obtain the full Green’s function matrix, an acoustic source (loudspeaker) is sequentially excited at each cavity site, and the acoustic pressure is measured in all cavities using microphones. This procedure is systematically repeated for every site across the entire lattice. The complex-valued energy spectra as well as left and right eigenstates of NH acoustic Chern insulators are obtained based on the method proposed in Ref. [1].

## S2.2 Acoustic cavities and tuning of onsite potentials

Figure S3 shows the tuning process of the onsite potentials of acoustic cavities. The acoustic cavities used in this study were fabricated using 3D printing with a tolerance of 0.2 mm or within 0.3%. The material is LEDO 6060 photosensitive resin, which behaves as acoustically rigid for airborne sound. Each printed cavity has a wall thickness of 6 mm. As shown in

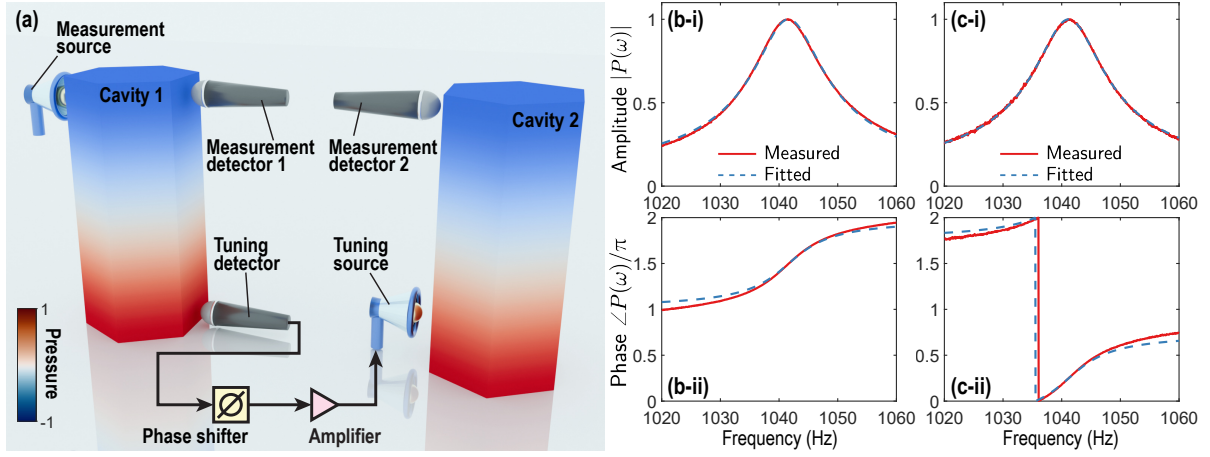

**Figure S4: Tuning hoppings between two acoustic cavities.** (a) Schematic illustration of the unidirectional hopping implemented using a detector and a source. The bottom microphone (tuning detector) in cavity 1 captures the acoustic pressure signal, which is processed by the controller to adjust its phase and amplitude before being emitted by the bottom loudspeaker (tuning source) in cavity 2. To determine both the amplitude and the phase of the unidirectional hopping  $\kappa_0$ , we excite at cavity 1 using a loudspeaker (measurement source) and measure the acoustic pressure in both cavities using two microphones (measurement detector). Experimentally measured and numerically fitted (i) amplitude and (ii) phase responses of the cross-power spectral density between the acoustic signals measured in cavities 1 and 2. For configuration (b), the target hopping strength is  $\kappa_0 = t_0/2 = 1.5 \text{ Hz}$ , and the retrieved value through fitting experimental results is  $\kappa_0 = 1.51 \text{ Hz} + 0.01i \text{ Hz}$ . For configuration (c), the target hopping strength is  $\kappa_0 = -h_y + ih_x = -0.3 \text{ Hz} + 0.3i \text{ Hz}$ , and the retrieved value through fitting experimental results is  $\kappa_0 = -0.303 \text{ Hz} + 0.302i \text{ Hz}$ .

Figs. S2 and S3, the cavities are hexagonal prisms with an interior height of  $l = 164 \text{ mm}$  and a side length of  $25 \text{ mm}$ . To characterize the cavity in the experiments, a loudspeaker (source) excites the cavity, and a microphone (detector) measures the acoustic pressure, as illustrated in Fig. S3(a). The onsite potential,  $\omega_0$ , of a cavity is retrieved using the Green's function for a single site:

$$G_0(\omega) = -\frac{\text{Im}(\omega_0)}{\omega - \omega_0}, \quad (\text{S8})$$

where  $\omega$  is the excitation frequency.

### S2.3 Tuning of hoppings

Figure S4 shows the tuning process of the hoppings. Both nonreciprocal and reciprocal hoppings between the cavities are implemented using detector-source (microphone-loudspeaker) pairs. In our platform, the hopping strength and phase are precisely controlled by a digital multi-channel controller, allowing flexible and reconfigurable manipulation of lattice hoppings. As illustrated in Fig. S4a, each unidirectional hopping is realized through a loudspeaker, a microphone, and an audio amplifier. The loudspeaker and microphone are positioned at the bottom of each cavity. The microphone captures the acoustic pressure signal, which is processed by the controller to adjust its phase and amplitude before being emitted by the loudspeaker in the

connected cavity. The analytical solution of this model is described in Sec. S2.4.

The tuning of the hopping parameters is performed as follows. As illustrated in Fig. S4a, a microphone is placed inside cavity 1 to detect the acoustic pressure. The detected pressure signal is then phase-adjusted, amplified, and emitted by the loudspeaker positioned in cavity 2. To determine both the amplitude and the phase of the unidirectional hopping  $\kappa_0$  in Eq. (S9), we excite at cavity 1 using a loudspeaker (measurement source in Fig. S4a) and measure the acoustic pressure in both cavities using two microphones (measurement detector in Fig. S4). The cross-power spectral density of these two measured pressure signals is expressed by Eq. (S13).

## S2.4 The coupled-model theory for the unidirectional coupling of two coupled acoustic cavities

Suppose two acoustic cavities (resonators) are connected by a unidirectional coupling  $\kappa_0$ . The tight-binding model Hamiltonian is

$$H_2 = \begin{pmatrix} \omega_0 & 0 \\ \kappa_0 & \omega_0 \end{pmatrix}. \quad (\text{S9})$$

Here,  $\text{Re}(\omega_0)$  is the first resonant (angular) frequency of a single cavity,  $-\text{Im}(\omega_0) > 0$  is the intrinsic loss, and  $\kappa_0$  is the unidirectional coupling realized by the active components. In general,  $\kappa_0 \in \mathbb{C}$  is a complex number.

Based on the coupled-mode theory, the dynamic equation for this system with a source excitation  $|s\rangle$  is

$$i \frac{d|\psi(t)\rangle}{dt} = H |\psi(t)\rangle + |s(t)\rangle, \quad (\text{S10})$$

where  $|\psi(t)\rangle = \begin{bmatrix} \psi_1(t) & \psi_2(t) \end{bmatrix}^T$  is the time-dependent sound pressure vector.

For a harmonic excitation at an angular frequency  $\omega$ , the excitation and sound pressure vectors can be written as  $|s(t)\rangle = |s\rangle e^{-i\omega t}$  and  $|\psi(t)\rangle = |\psi\rangle e^{-i\omega t}$ , respectively. The dynamic equation (S10) is then expressed as

$$(\omega - H_2) |\psi\rangle = |s\rangle. \quad (\text{S11})$$

When the source is excited at cavity 1, the excitation vector is  $|s\rangle = \psi_{\text{in}} \begin{bmatrix} 1 & 0 \end{bmatrix}^T$ , where  $\psi_{\text{in}}$  is the complex amplitude. Consequently, the sound pressure distribution is obtained by solving Eq. (S11) to give

$$|\psi(t)\rangle = \psi_{\text{in}} e^{-i\omega t} \begin{bmatrix} 1 & \kappa_0 \\ \omega - \omega_0 & (\omega - \omega_0)^2 \end{bmatrix}^T. \quad (\text{S12})$$

To determine the phase of the unidirectional coupling  $\kappa_0$ , the cross-power spectral density

between two measured signals is calculated in experiments

$$P(\omega) \equiv \frac{\psi_2(\omega)}{\psi_1(\omega)} = \frac{\kappa_0}{\omega - \omega_0}. \quad (\text{S13})$$

It is observed that, when  $\omega = \text{Re}(\omega_0)$ , the phase of  $P$  and  $\kappa_0$  follows the relation

$$\angle P(\text{Re}(\omega_0)) = \angle \kappa_0 - \frac{\pi}{2}. \quad (\text{S14})$$

### S3 Extended experimental results

In this section of the Supplemental Material, we display additional results from our experimental measurements and their comparison with theoretical predictions. The outcomes are summarized in Table 1 and the results are explicitly displayed in Figs. S5-S56. While discussing the results we will be using a few abbreviations. So, we announce them up front. Specifically, NH stands for non-Hermitian, PBCs stand for periodic boundary conditions, OBCs stand for open boundary conditions, NHDS stands for non-Hermitian dislocation states, and D-NHSE stands for dislocation induced non-Hermitian skin effect.

**Table 1:** Figure references of the extended experimental results. Parameters are  $\omega_0 = 1040\text{Hz} - 4.5i\text{Hz}$  and  $t_0 = 3\text{Hz}$ .

| Figure label | Boundary condition | $m_0/t_0$ | $h_x/t_0$ | $h_y/t_0$ | $h_z/t_0$ | Comment                                                                                               |
|--------------|--------------------|-----------|-----------|-----------|-----------|-------------------------------------------------------------------------------------------------------|
| S5           | PBC                | -1        | 0         | 0         | 0         | Zero-energy dislocation bound states.                                                                 |
| S6           | OBC                | -1        | 0         | 0         | 0         | Zero-energy dislocation bound states. Boundary states.                                                |
| S7           | PBC                | 1         | 0         | 0         | 0         | No dislocation bound states.                                                                          |
| S8           | OBC                | 1         | 0         | 0         | 0         | No dislocation bound states. Mid-gap boundary states.                                                 |
| S9           | PBC                | -1        | 0.3       | 0         | 0         | Zero-energy NHDSs. Asymmetric NHDS distribution along $x$ direction. No D-NHSE.                       |
| S10          | OBC                | -1        | 0.3       | 0         | 0         | Zero-energy NHDSs. Asymmetric NHDS distribution along $x$ direction. NHSE along $x$ direction.        |
| S11          | PBC                | 1         | 0.3       | 0         | 0         | No NHDS. No D-NHSE.                                                                                   |
| S12          | OBC                | 1         | 0.3       | 0         | 0         | No NHDS. NHSE along $x$ direction.                                                                    |
| S13          | PBC                | -1        | 0.6       | 0         | 0         | Zero-energy NHDS. No D-NHSE.                                                                          |
| S14          | OBC                | -1        | 0.6       | 0         | 0         | Zero-energy NHDS. Asymmetric NHDS distribution along $x$ direction. NHSE along $x$ direction.         |
| S15          | PBC                | 1         | 0.6       | 0         | 0         | No NHDS. No D-NHSE.                                                                                   |
| S16          | OBC                | 1         | 0.6       | 0         | 0         | No NHDS. NHSE along $x$ direction.                                                                    |
| S17          | PBC                | -1        | 0.9       | 0         | 0         | Zero-energy NHDS with weights at the dislocation cores start to show signs of diminishing. No D-NHSE. |

*Continued on next page*

| Figure label | Boundary condition | $m_0/t_0$ | $h_x/t_0$ | $h_y/t_0$ | $h_z/t_0$ | Comment                                                                                                                                                                 |
|--------------|--------------------|-----------|-----------|-----------|-----------|-------------------------------------------------------------------------------------------------------------------------------------------------------------------------|
| S18          | OBC                | -1        | 0.9       | 0         | 0         | Zero-energy NHDSs with weights at the dislocation cores start to show signs of diminishing. Asymmetric NHDS distribution along $x$ direction. NHSE along $x$ direction. |
| S19          | PBC                | 1         | 0.9       | 0         | 0         | No NHDS. No D-NHSE.                                                                                                                                                     |
| S20          | OBC                | 1         | 0.9       | 0         | 0         | No NHDS. NHSE along $x$ direction.                                                                                                                                      |
| S21          | PBC                | -1        | 1.1       | 0         | 0         | No NHDS. No D-NHSE.                                                                                                                                                     |
| S22          | OBC                | -1        | 1.1       | 0         | 0         | No NHDS. NHSE along $x$ direction.                                                                                                                                      |
| S23          | PBC                | 1         | 1.1       | 0         | 0         | No NHDS. No D-NHSE.                                                                                                                                                     |
| S24          | OBC                | 1         | 1.1       | 0         | 0         | No NHDS. NHSE along $x$ direction.                                                                                                                                      |
| S25          | PBC                | -1        | 0         | 0.3       | 0         | NHDS. D-NHSE along $y$ direction.                                                                                                                                       |
| S26          | OBC                | -1        | 0         | 0.3       | 0         | Slightly delocalized NHDS. NHSE along $y$ direction.                                                                                                                    |
| S27          | PBC                | 1         | 0         | 0.3       | 0         | No NHDS. D-NHSE along $y$ direction.                                                                                                                                    |
| S28          | OBC                | 1         | 0         | 0.3       | 0         | No NHDS. NHSE along $y$ direction.                                                                                                                                      |
| S29          | PBC                | -1        | 0         | 0.6       | 0         | NHDS. D-NHSE along $y$ direction.                                                                                                                                       |
| S30          | OBC                | -1        | 0         | 0.6       | 0         | Slightly delocalized NHDS. NHSE along $y$ direction.                                                                                                                    |
| S31          | PBC                | 1         | 0         | 0.6       | 0         | No NHDS. D-NHSE along $y$ direction.                                                                                                                                    |
| S32          | OBC                | 1         | 0         | 0.6       | 0         | No NHDS. NHSE along $y$ direction.                                                                                                                                      |
| S33          | PBC                | -1        | 0         | 0.9       | 0         | NHDS. D-NHSE along $y$ direction.                                                                                                                                       |
| S34          | OBC                | -1        | 0         | 0.9       | 0         | Substantially delocalized NHDS. NHSE along $y$ direction.                                                                                                               |
| S35          | PBC                | 1         | 0         | 0.9       | 0         | No NHDS. D-NHSE along $y$ direction.                                                                                                                                    |
| S36          | OBC                | 1         | 0         | 0.9       | 0         | No NHDS. NHSE along $y$ direction.                                                                                                                                      |
| S37          | PBC                | -1        | 0         | 1.1       | 0         | No NHDS. D-NHSE along $y$ direction.                                                                                                                                    |
| S38          | OBC                | -1        | 0         | 1.1       | 0         | No NHDS. NHSE along $y$ direction.                                                                                                                                      |
| S39          | PBC                | 1         | 0         | 1.1       | 0         | No NHDS. D-NHSE along $y$ direction.                                                                                                                                    |
| S40          | OBC                | 1         | 0         | 1.1       | 0         | No NHDS. NHSE along $y$ direction.                                                                                                                                      |
| S41          | PBC                | -1        | 0         | 0         | 0.3       | NHDS. No D-NHSE.                                                                                                                                                        |
| S42          | OBC                | -1        | 0         | 0         | 0.3       | NHDS. Boundary states. No NHSE.                                                                                                                                         |
| S43          | PBC                | 1         | 0         | 0         | 0.3       | No NHDS. No D-NHSE.                                                                                                                                                     |
| S44          | OBC                | 1         | 0         | 0         | 0.3       | No NHDS. Boundary states. No NHSE.                                                                                                                                      |
| S45          | PBC                | -1        | 0         | 0         | 0.6       | NHDS. No D-NHSE.                                                                                                                                                        |

*Continued on next page*

| Figure label | Boundary condition | $m_0/t_0$ | $h_x/t_0$ | $h_y/t_0$ | $h_z/t_0$ | Comment                                                 |
|--------------|--------------------|-----------|-----------|-----------|-----------|---------------------------------------------------------|
| S46          | OBC                | -1        | 0         | 0         | 0.6       | Slightly delocalized NHDS and boundary states. No NHSE. |
| S47          | PBC                | 1         | 0         | 0         | 0.6       | No NHDS. No D-NHSE.                                     |
| S48          | OBC                | 1         | 0         | 0         | 0.6       | No NHDS. No NHSE.                                       |
| S49          | PBC                | -1        | 0         | 0         | 0.9       | NHDS. No D-NHSE.                                        |
| S50          | OBC                | -1        | 0         | 0         | 0.9       | Substantially delocalized NHDS. No NHSE.                |
| S51          | PBC                | 1         | 0         | 0         | 0.9       | No NHDS. No D-NHSE.                                     |
| S52          | OBC                | 1         | 0         | 0         | 0.9       | No NHDS. No NHSE.                                       |
| S53          | PBC                | -1        | 0         | 0         | 1.1       | No NHDS. No D-NHSE.                                     |
| S54          | OBC                | -1        | 0         | 0         | 1.1       | No NHDS. No NHSE.                                       |
| S55          | PBC                | 1         | 0         | 0         | 1.1       | No NHDS. No D-NHSE.                                     |
| S56          | OBC                | 1         | 0         | 0         | 1.1       | No NHDS. No NHSE.                                       |

*End of table*

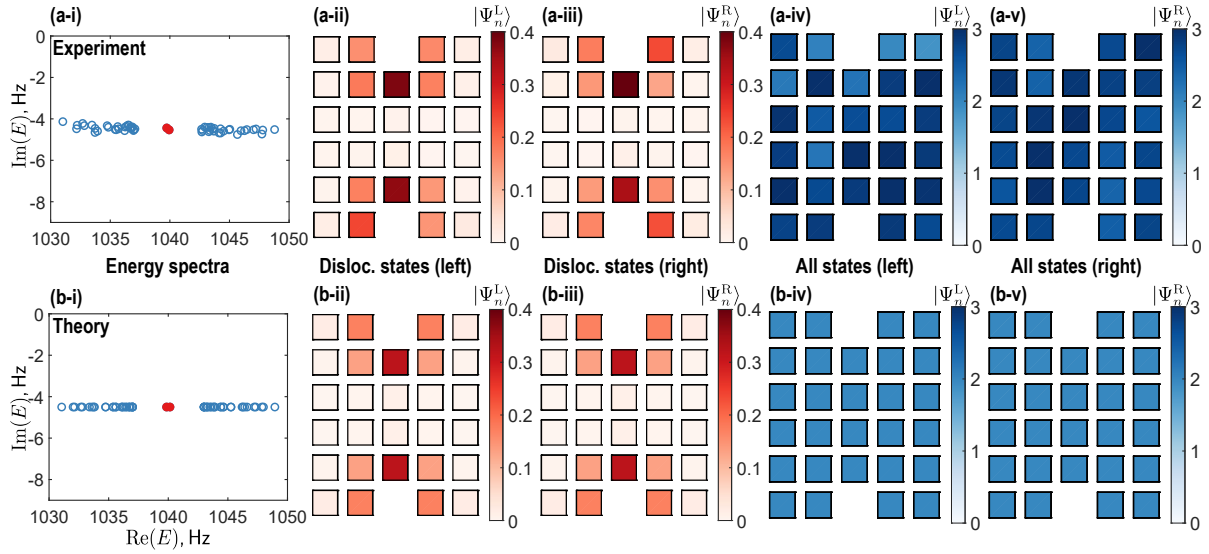

**Figure S5:** (a) Experimental results and (b) theoretical predictions of Hermitian acoustic Chern insulators with an edge dislocation-antidislocation pair under PBCs in the M phase. (i) Energy spectra. Red dots ●, dislocation states; Blue circles ○, other states. Amplitude distributions of the (ii) left and (iii) right eigenstates for the dislocation states. Summed amplitude distributions of all (iv) left and (v) right eigenstates. Parameters:  $\omega_0 = 1040 \text{ Hz} - 4.5i \text{ Hz}$ ,  $t_0 = -m_0 = 3 \text{ Hz}$ ,  $h_x = h_y = h_z = 0$ .

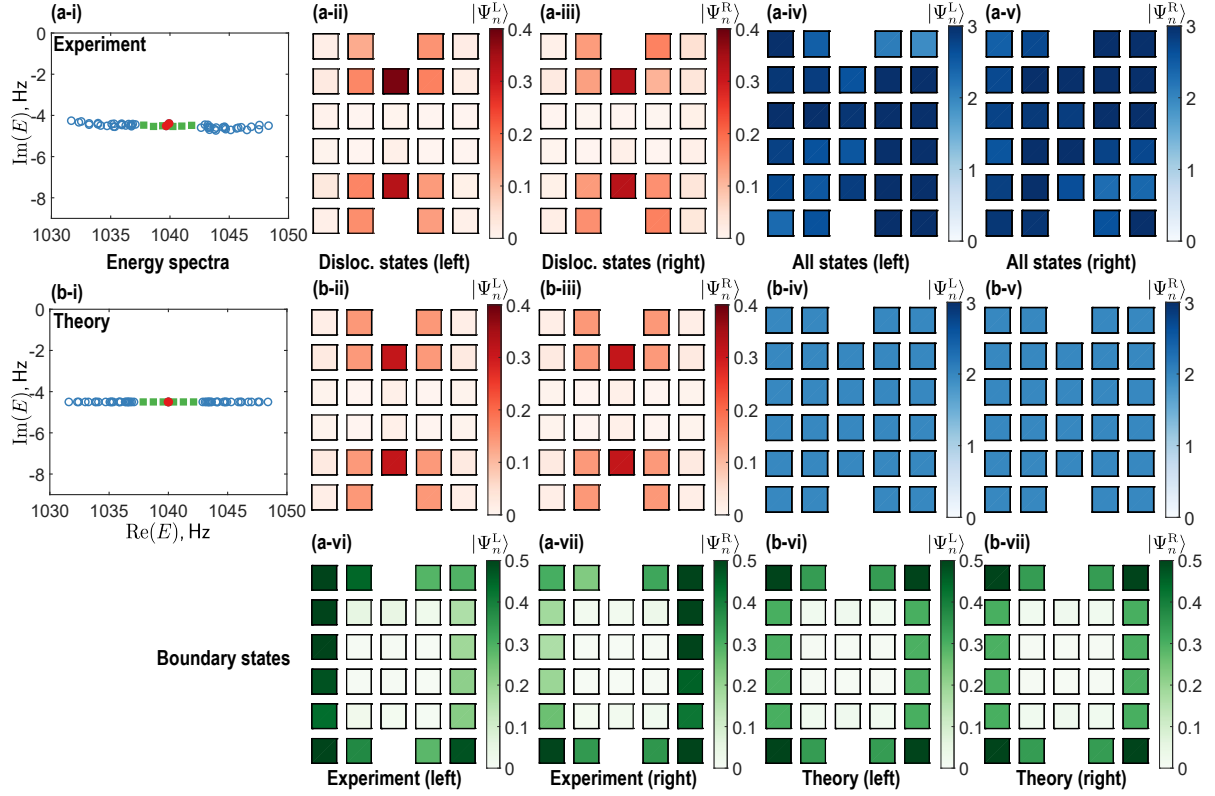

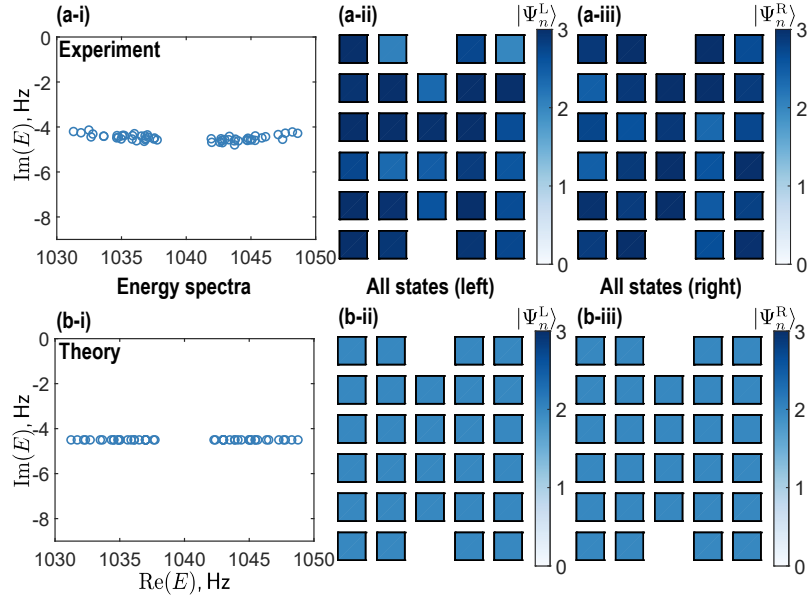

**Figure S7:** (a) Experimental results and (b) theoretical predictions of Hermitian acoustic Chern insulators with an edge dislocation-antidislocation pair under PBCs in the  $\Gamma$  phase. (i) Energy spectra. Summed amplitude distributions of all (ii) left and (iii) right eigenstates. Parameters:  $\omega_0 = 1040\text{Hz} - 4.5i\text{Hz}$ ,  $t_0 = m_0 = 3\text{Hz}$ ,  $h_x = h_y = h_z = 0$ .

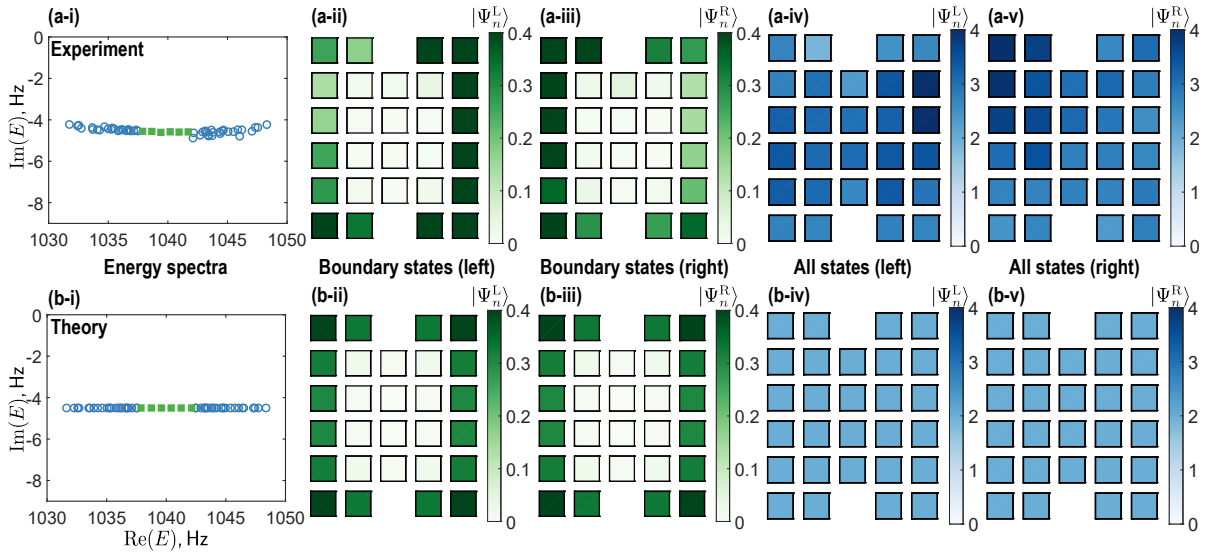

**Figure S8:** (a) Experimental results and (b) theoretical predictions of Hermitian acoustic Chern insulators with an edge dislocation-antidislocation pair under OBCs in the  $\Gamma$  phase. (i) Energy spectra. Green squares ■, boundary states; Blue circles ○, other states. Amplitude distributions of the (ii) left and (iii) right eigenstates for the boundary states. Summed amplitude distributions of all (iv) left and (v) right eigenstates. Parameters:  $\omega_0 = 1040\text{Hz} - 4.5i\text{Hz}$ ,  $t_0 = m_0 = 3\text{Hz}$ ,  $h_x = h_y = h_z = 0$ .

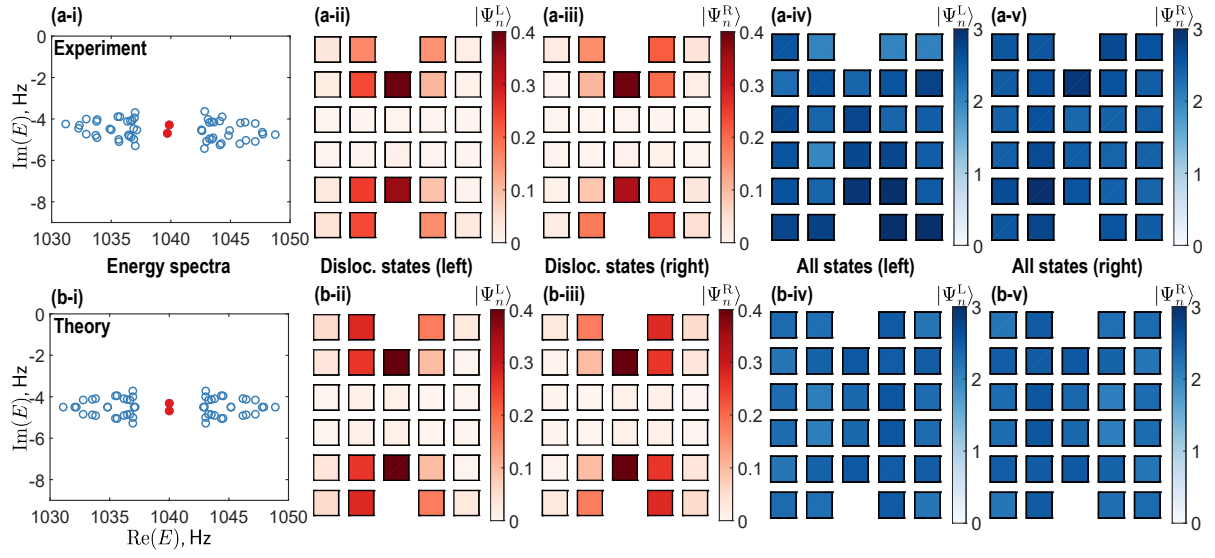

**Figure S9:** (a) Experimental results and (b) theoretical predictions of NH acoustic Chern insulators with an edge dislocation-antidislocation pair under PBCs in the M phase. (i) Energy spectra. Red dots ●, dislocation states; Blue circles ○, other states. Amplitude distributions of the (ii) left and (iii) right eigenstates for the NHDSs. Summed amplitude distributions of all (iv) left and (v) right eigenstates. Parameters:  $\omega_0 = 1040 \text{ Hz} - 4.5i \text{ Hz}$ ,  $t_0 = -m_0 = 3 \text{ Hz}$ ,  $h_x = 0.9 \text{ Hz}$ ,  $h_y = h_z = 0$ .

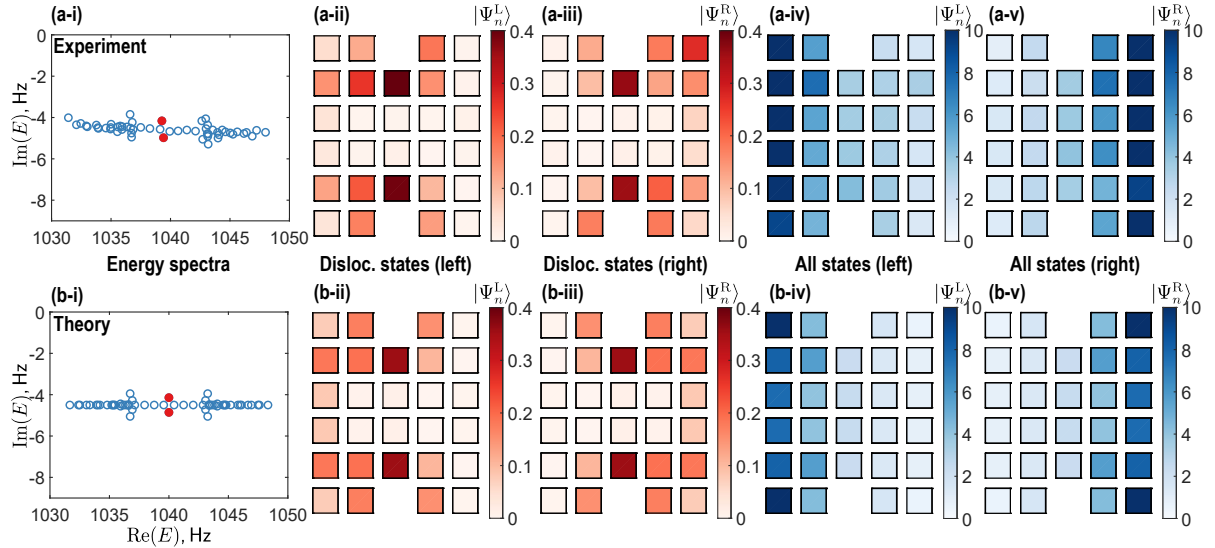

**Figure S10:** (a) Experimental results and (b) theoretical predictions of NH acoustic Chern insulators with an edge dislocation-antidislocation pair under OBCs in the M phase. (i) Energy spectra. Red dots ●, dislocation states; blue circles ○, all other states. Amplitude distributions of the (ii) left and (iii) right eigenstates for the dislocation states. Summed amplitude distributions of all (iv) left and (v) right eigenstates. Parameters:  $\omega_0 = 1040 \text{ Hz} - 4.5i \text{ Hz}$ ,  $t_0 = -m_0 = 3 \text{ Hz}$ ,  $h_x = 0.9 \text{ Hz}$ ,  $h_y = h_z = 0$ .

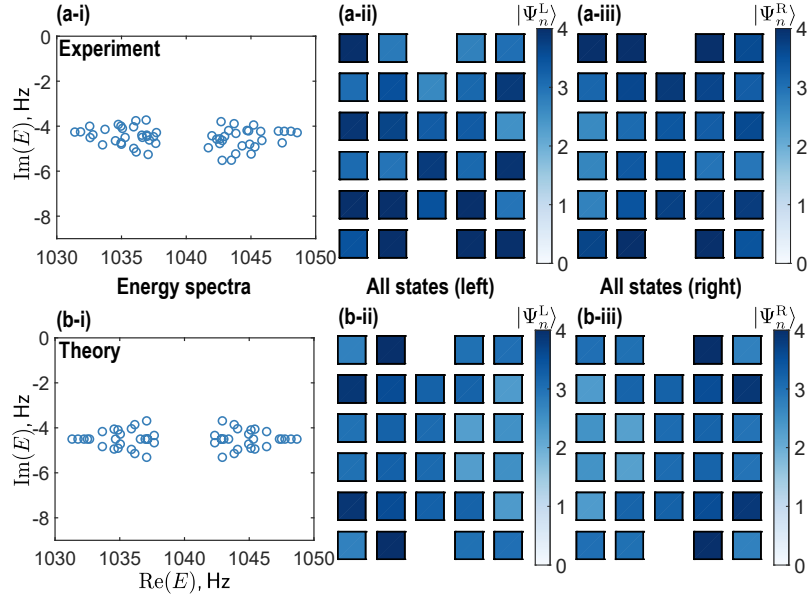

**Figure S11:** (a) Experimental results and (b) theoretical predictions of NH acoustic Chern insulators with an edge dislocation-antidislocation pair under PBCs in the  $\Gamma$  phase. (i) Energy spectra. Summed amplitude distributions of all (ii) left and (iii) right eigenstates. Parameters:  $\omega_0 = 1040\text{ Hz} - 4.5i\text{ Hz}$ ,  $t_0 = m_0 = 3\text{ Hz}$ ,  $h_x = 0.9\text{ Hz}$ ,  $h_y = h_z = 0$ .

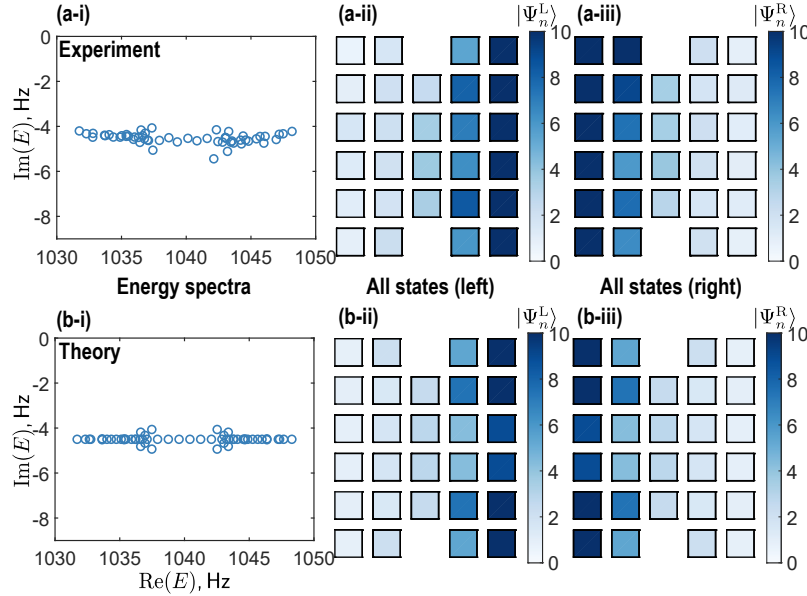

**Figure S12:** (a) Experimental results and (b) theoretical predictions of NH acoustic Chern insulators with an edge dislocation-antidislocation pair under OBCs in the  $\Gamma$  phase. (i) Energy spectra. Summed amplitude distributions of all (ii) left and (iii) right eigenstates. Parameters:  $\omega_0 = 1040\text{ Hz} - 4.5i\text{ Hz}$ ,  $t_0 = m_0 = 3\text{ Hz}$ ,  $h_x = 0.9\text{ Hz}$ ,  $h_y = h_z = 0$ .

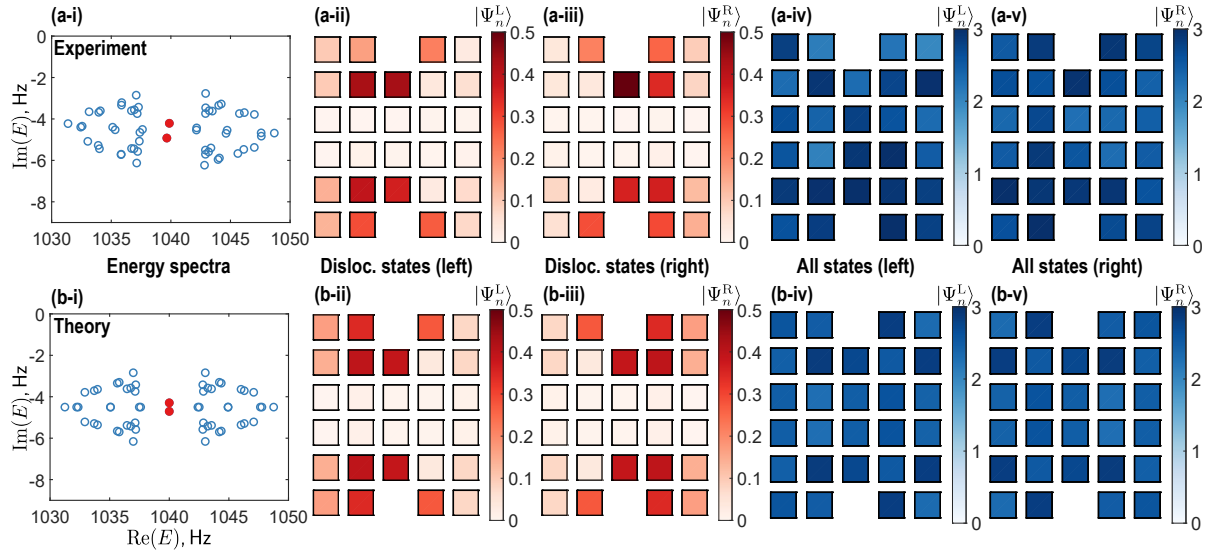

**Figure S13:** (a) Experimental results and (b) theoretical predictions of NH acoustic Chern insulators with an edge dislocation-antidislocation pair under PBCs in the M phase. (i) Energy spectra. Red dots  $\bullet$ , dislocation states; Blue circles  $\circ$ , other states. Amplitude distributions of the (ii) left and (iii) right eigenstates for the NHDSs. Summed amplitude distributions of all (iv) left and (v) right eigenstates. Parameters:  $\omega_0 = 1040\text{Hz} - 4.5i\text{Hz}$ ,  $t_0 = -m_0 = 3\text{Hz}$ ,  $h_x = 1.8\text{Hz}$ ,  $h_y = h_z = 0$ .

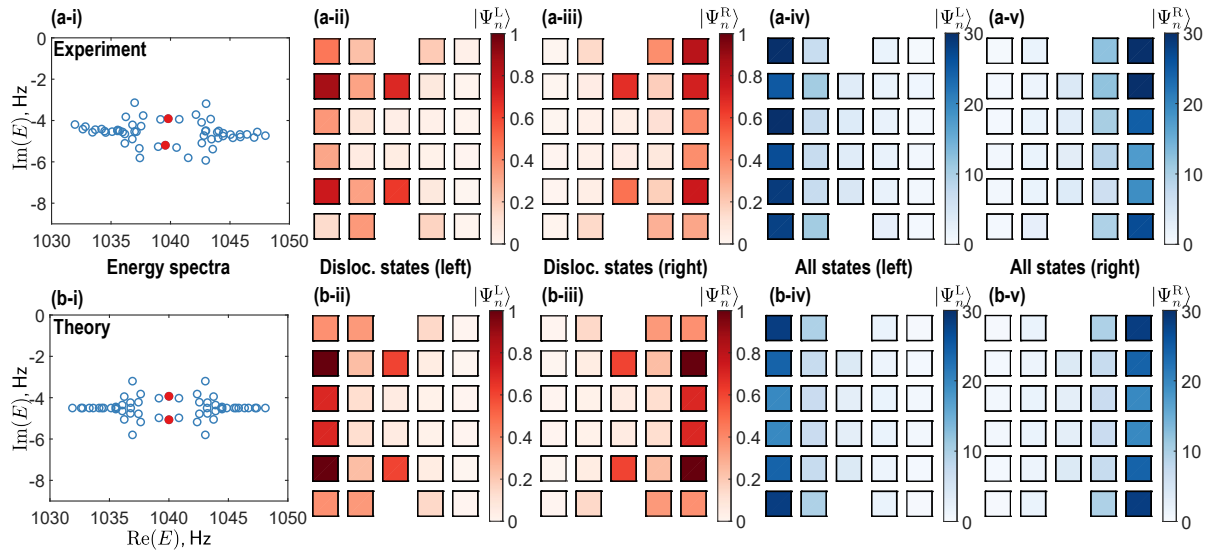

**Figure S14:** (a) Experimental results and (b) theoretical predictions of NH acoustic Chern insulators with an edge dislocation-antidislocation pair under OBCs in the M phase. (i) Energy spectra. Red dots  $\bullet$ , dislocation states; Blue circles  $\circ$ , other states. Amplitude distributions of the (ii) left and (iii) right eigenstates for the NHDSs. Summed amplitude distributions of all (iv) left and (v) right eigenstates. Parameters:  $\omega_0 = 1040\text{Hz} - 4.5i\text{Hz}$ ,  $t_0 = -m_0 = 3\text{Hz}$ ,  $h_x = 1.8\text{Hz}$ ,  $h_y = h_z = 0$ .

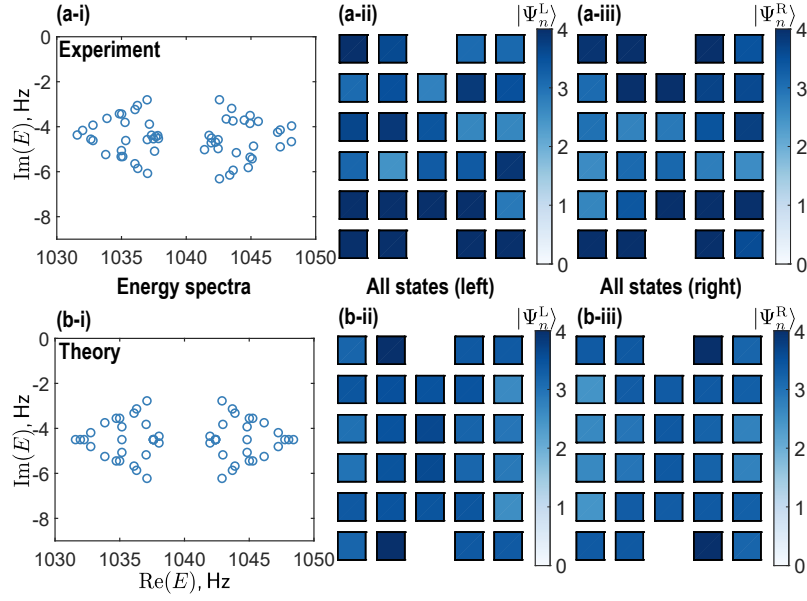

**Figure S15:** (a) Experimental results and (b) theoretical predictions of NH acoustic Chern insulators with an edge dislocation-antidislocation pair under PBCs in the  $\Gamma$  phase. (i) Energy spectra. Summed amplitude distributions of all (ii) left and (iii) right eigenstates. Parameters:  $\omega_0 = 1040 \text{ Hz} - 4.5i \text{ Hz}$ ,  $t_0 = m_0 = 3 \text{ Hz}$ ,  $h_x = 1.8 \text{ Hz}$ ,  $h_y = h_z = 0$ .

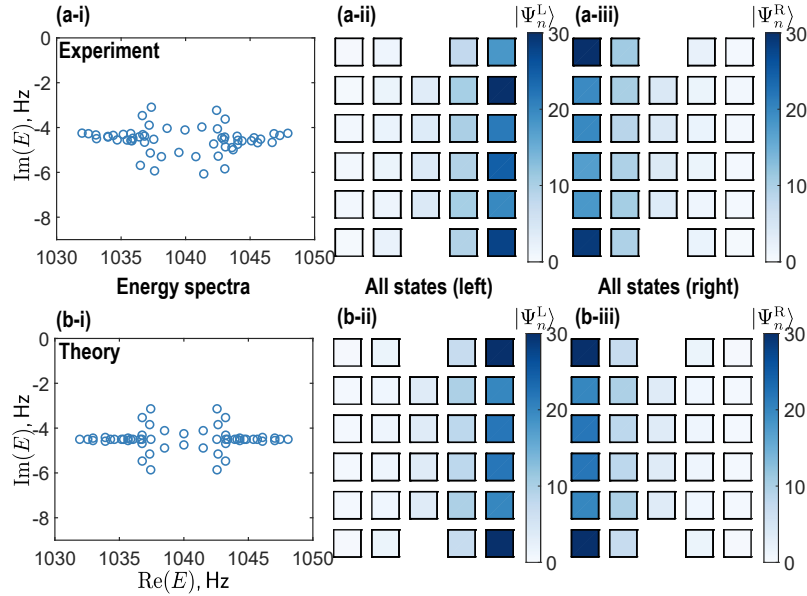

**Figure S16:** (a) Experimental results and (b) theoretical predictions of NH acoustic Chern insulators with an edge dislocation-antidislocation pair under OBCs in the  $\Gamma$  phase. (i) Energy spectra. Summed amplitude distributions of all (ii) left and (iii) right eigenstates. Parameters:  $\omega_0 = 1040 \text{ Hz} - 4.5i \text{ Hz}$ ,  $t_0 = m_0 = 3 \text{ Hz}$ ,  $h_x = 1.8 \text{ Hz}$ ,  $h_y = h_z = 0$ .

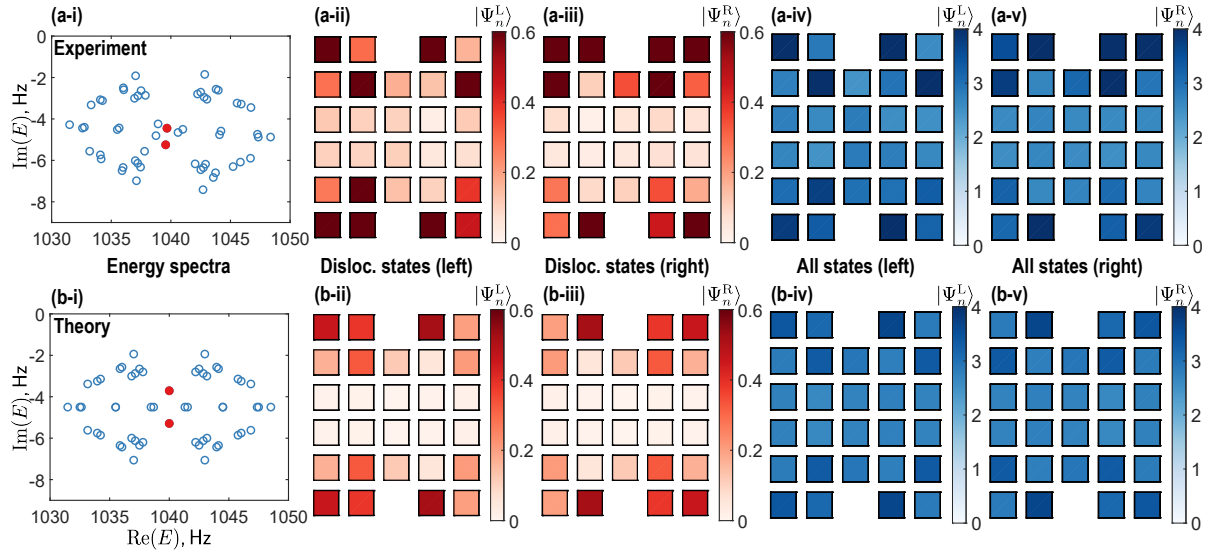

**Figure S17:** (a) Experimental results and (b) theoretical predictions of NH acoustic Chern insulators with an edge dislocation-antidislocation pair under PBCs in the M phase. (i) Energy spectra. Red dots ●, dislocation states; Blue circles ○, other states. Amplitude distributions of the (ii) left and (iii) right eigenstates for the NHDSs. Summed amplitude distributions of all (iv) left and (v) right eigenstates. Parameters:  $\omega_0 = 1040 \text{ Hz} - 4.5i \text{ Hz}$ ,  $t_0 = -m_0 = 3 \text{ Hz}$ ,  $h_x = 2.7 \text{ Hz}$ ,  $h_y = h_z = 0$ .

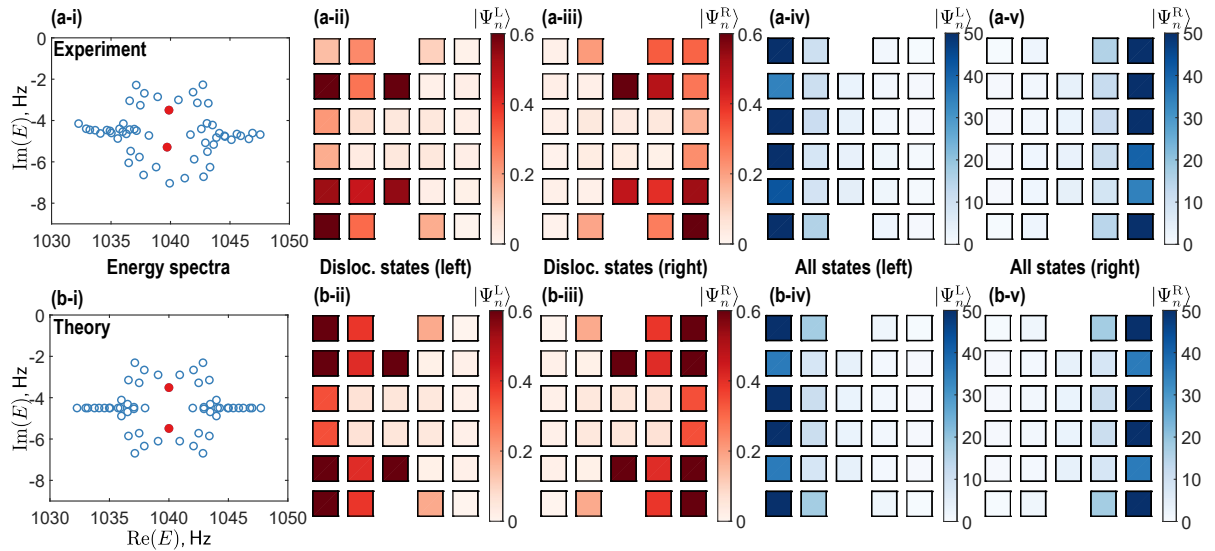

**Figure S18:** (a) Experimental results and (b) theoretical predictions of NH acoustic Chern insulators with an edge dislocation-antidislocation pair under OBCs in the M phase. (i) Energy spectra. Red dots ●, dislocation states; Blue circles ○, other states. Amplitude distributions of the (ii) left and (iii) right eigenstates for the NHDSs. Summed amplitude distributions of all (iv) left and (v) right eigenstates. Parameters:  $\omega_0 = 1040 \text{ Hz} - 4.5i \text{ Hz}$ ,  $t_0 = -m_0 = 3 \text{ Hz}$ ,  $h_x = 2.7 \text{ Hz}$ ,  $h_y = h_z = 0$ .

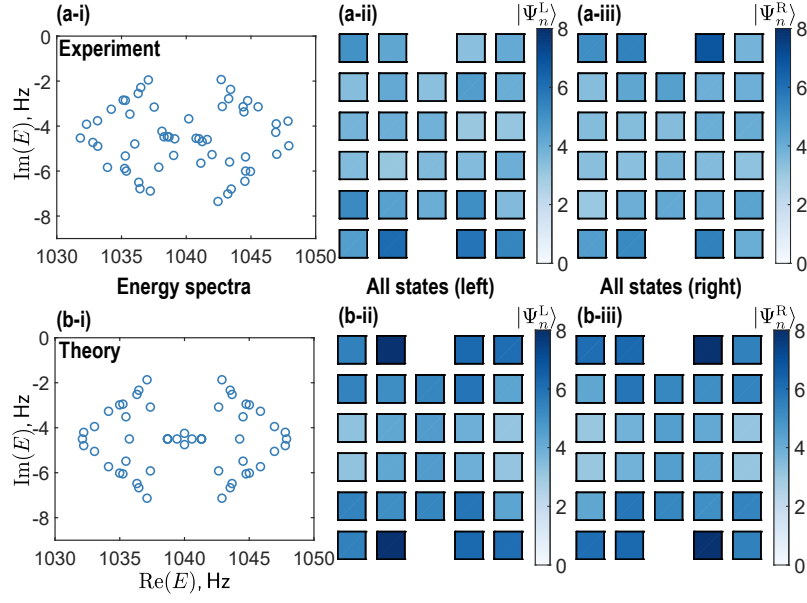

**Figure S19:** (a) Experimental results and (b) theoretical predictions of NH acoustic Chern insulators with an edge dislocation-antidislocation pair under PBCs in the  $\Gamma$  phase. (i) Energy spectra. Summed amplitude distributions of all (ii) left and (iii) right eigenstates. Parameters:  $\omega_0 = 1040 \text{ Hz} - 4.5i \text{ Hz}$ ,  $t_0 = m_0 = 3 \text{ Hz}$ ,  $h_x = 2.7 \text{ Hz}$ ,  $h_y = h_z = 0$ .

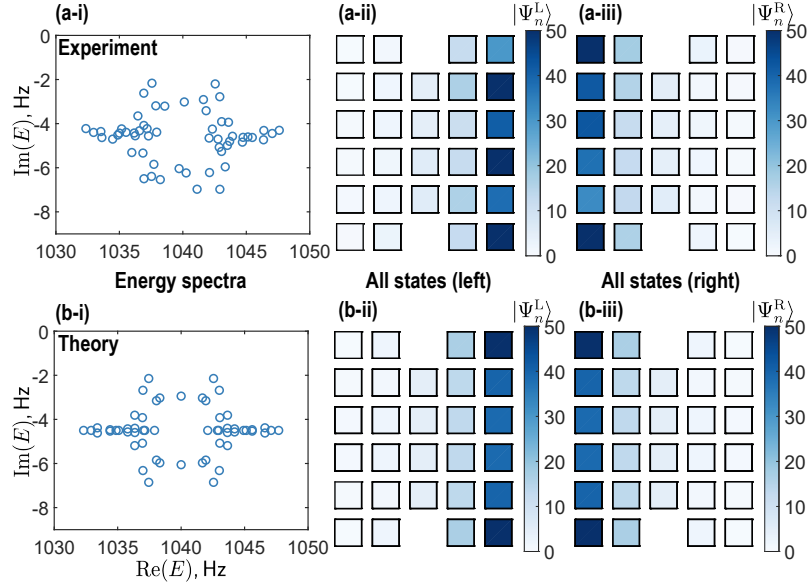

**Figure S20:** (a) Experimental results and (b) theoretical predictions of NH acoustic Chern insulators with an edge dislocation-antidislocation pair under OBCs in the  $\Gamma$  phase. (i) Energy spectra. Summed amplitude distributions of all (ii) left and (iii) right eigenstates. Parameters:  $\omega_0 = 1040 \text{ Hz} - 4.5i \text{ Hz}$ ,  $t_0 = m_0 = 3 \text{ Hz}$ ,  $h_x = 2.7 \text{ Hz}$ ,  $h_y = h_z = 0$ .

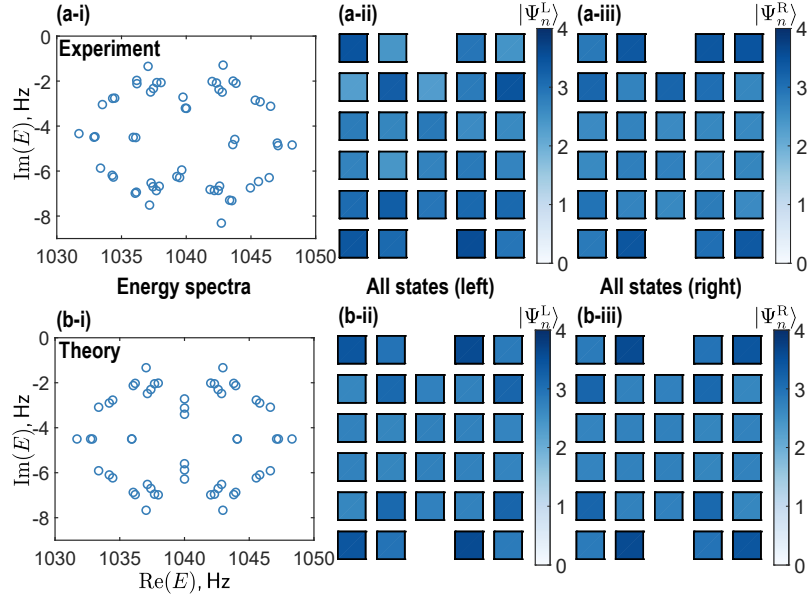

**Figure S21:** (a) Experimental results and (b) theoretical predictions of NH acoustic Chern insulators with an edge dislocation-antidislocation pair under PBCs in the M phase. (i) Energy spectra. Summed amplitude distributions of all (ii) left and (iii) right eigenstates. Parameters:  $\omega_0 = 1040\text{ Hz} - 4.5i\text{ Hz}$ ,  $t_0 = -m_0 = 3\text{ Hz}$ ,  $h_x = 3.3\text{ Hz}$ ,  $h_y = h_z = 0$ .

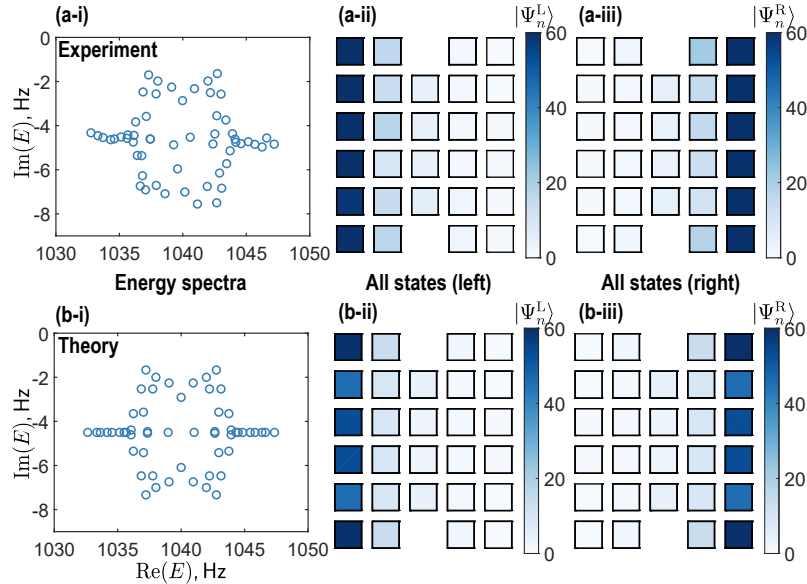

**Figure S22:** (a) Experimental results and (b) theoretical predictions of NH acoustic Chern insulators with an edge dislocation-antidislocation pair under PBCs in the M phase. (i) Energy spectra. Summed amplitude distributions of all (ii) left and (iii) right eigenstates. Parameters:  $\omega_0 = 1040\text{ Hz} - 4.5i\text{ Hz}$ ,  $t_0 = -m_0 = 3\text{ Hz}$ ,  $h_x = 3.3\text{ Hz}$ ,  $h_y = h_z = 0$ .

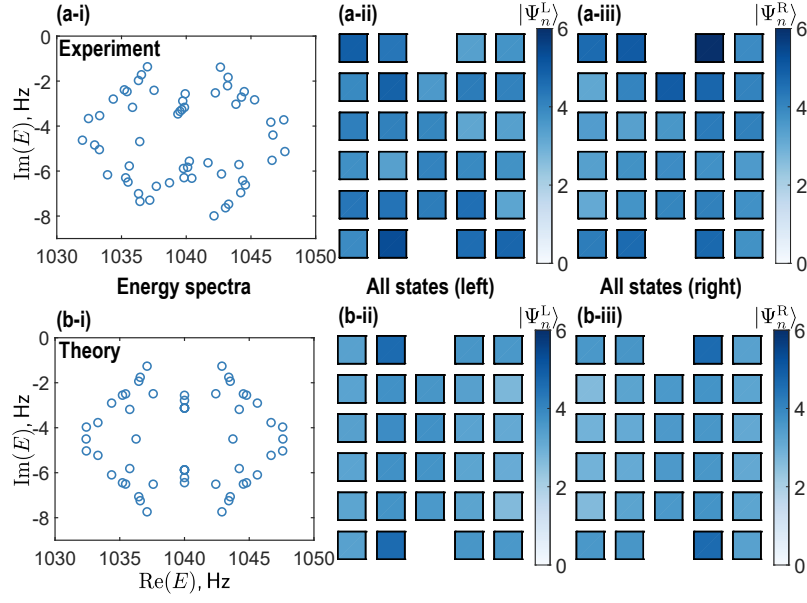

**Figure S23:** (a) Experimental results and (b) theoretical predictions of NH acoustic Chern insulators with an edge dislocation-antidislocation pair under PBCs in the  $\Gamma$  phase. (i) Energy spectra. Summed amplitude distributions of all (ii) left and (iii) right eigenstates. Parameters:  $\omega_0 = 1040 \text{ Hz} - 4.5i \text{ Hz}$ ,  $t_0 = m_0 = 3 \text{ Hz}$ ,  $h_x = 3.3 \text{ Hz}$ ,  $h_y = h_z = 0$ .

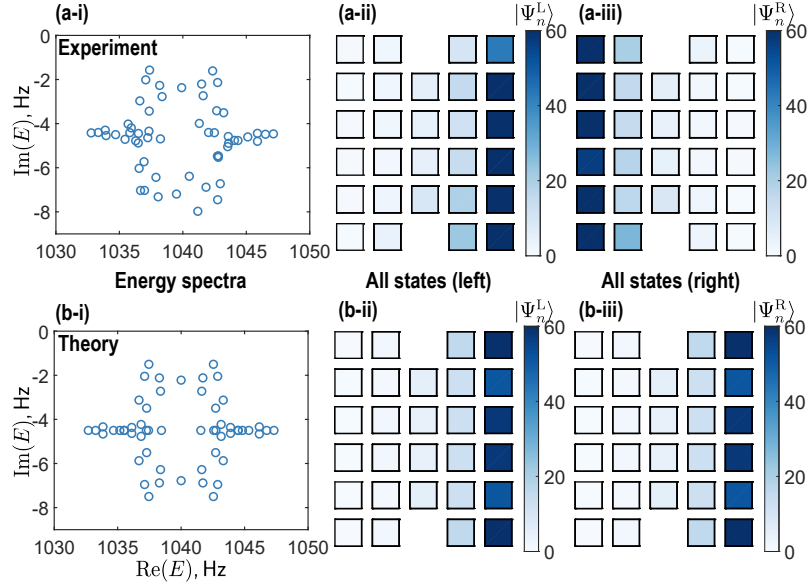

**Figure S24:** (a) Experimental results and (b) theoretical predictions of NH acoustic Chern insulators with an edge dislocation-antidislocation pair under PBCs in the  $\Gamma$  phase. (i) Energy spectra. Summed amplitude distributions of all (ii) left and (iii) right eigenstates. Parameters:  $\omega_0 = 1040 \text{ Hz} - 4.5i \text{ Hz}$ ,  $t_0 = m_0 = 3 \text{ Hz}$ ,  $h_x = 3.3 \text{ Hz}$ ,  $h_y = h_z = 0$ .

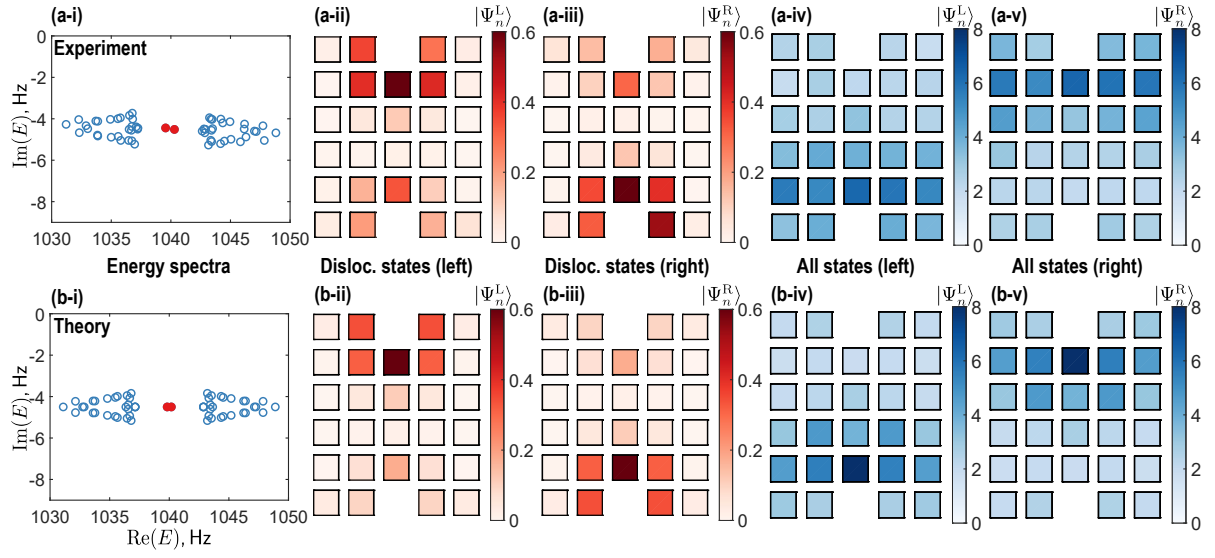

**Figure S25:** (a) Experimental results and (b) theoretical predictions of NH acoustic Chern insulators with an edge dislocation-antidislocation pair under PBCs in the M phase. (i) Energy spectra. Red dots ●, dislocation states; Blue circles ○, other states. Amplitude distributions of the (ii) left and (iii) right eigenstates for the NHDSs. Summed amplitude distributions of all (iv) left and (v) right eigenstates. Parameters:  $\omega_0 = 1040\text{Hz} - 4.5i\text{Hz}$ ,  $t_0 = -m_0 = 3\text{Hz}$ ,  $h_y = 0.9\text{Hz}$ ,  $h_x = h_z = 0$ .

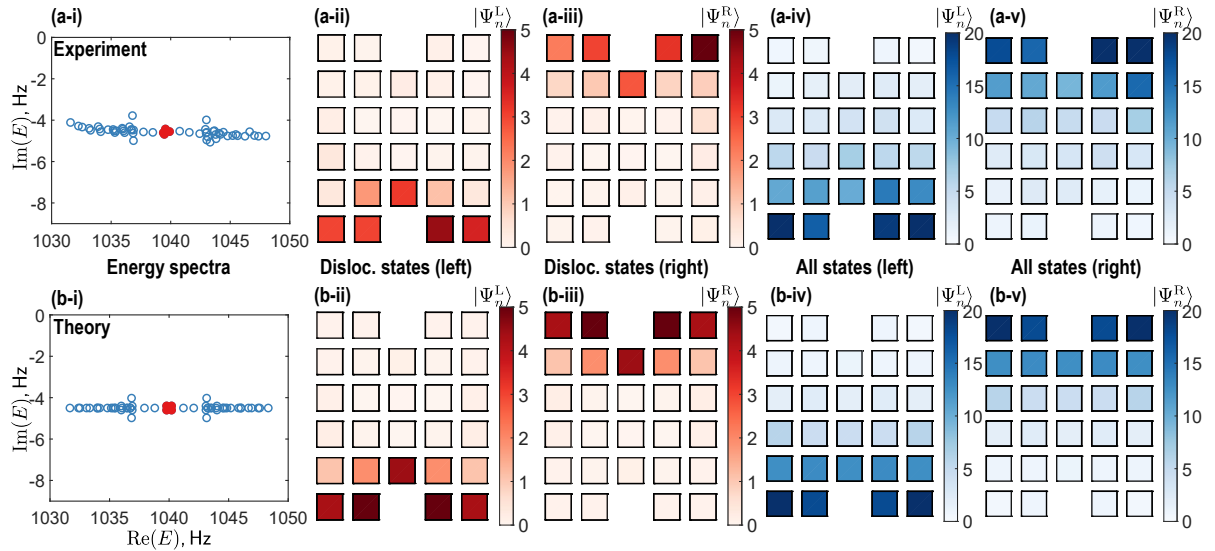

**Figure S26:** (a) Experimental results and (b) theoretical predictions of NH acoustic Chern insulators with an edge dislocation-antidislocation pair under OBCs in the M phase. (i) Energy spectra. Red dots ●, dislocation states; Blue circles ○, other states. Summed amplitude distributions of the (ii) left and (iii) right eigenstates for the NHDS. Summed amplitude distributions of all (iv) left and (v) right eigenstates. Parameters:  $\omega_0 = 1040\text{Hz} - 4.5i\text{Hz}$ ,  $t_0 = -m_0 = 3\text{Hz}$ ,  $h_y = 0.9\text{Hz}$ ,  $h_x = h_z = 0$ .

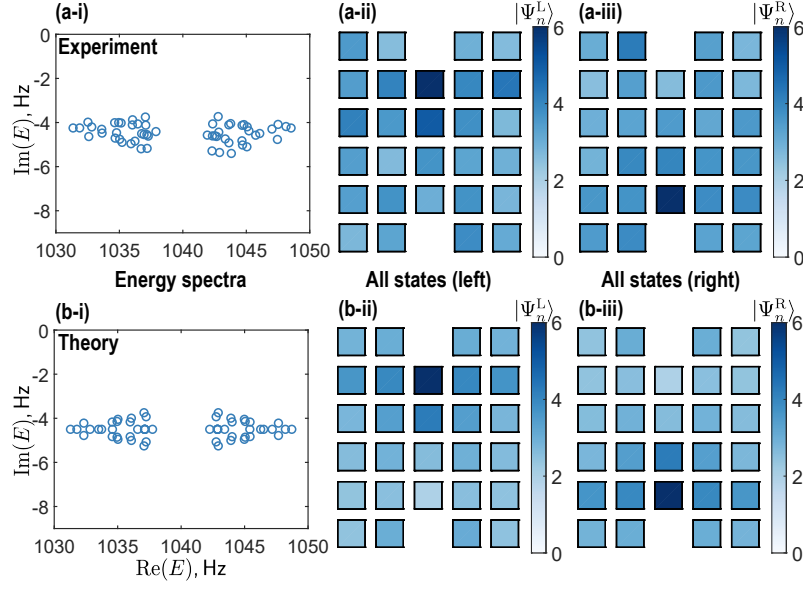

**Figure S27:** (a) Experimental results and (b) theoretical predictions of NH acoustic Chern insulators with an edge dislocation-antidislocation pair under PBCs in the  $\Gamma$  phase. (i) Energy spectra. Summed amplitude distributions of all (ii) left and (iii) right eigenstates. Parameters:  $\omega_0 = 1040\text{ Hz} - 4.5i\text{ Hz}$ ,  $t_0 = m_0 = 3\text{ Hz}$ ,  $h_y = 0.9\text{ Hz}$ ,  $h_x = h_z = 0$ .

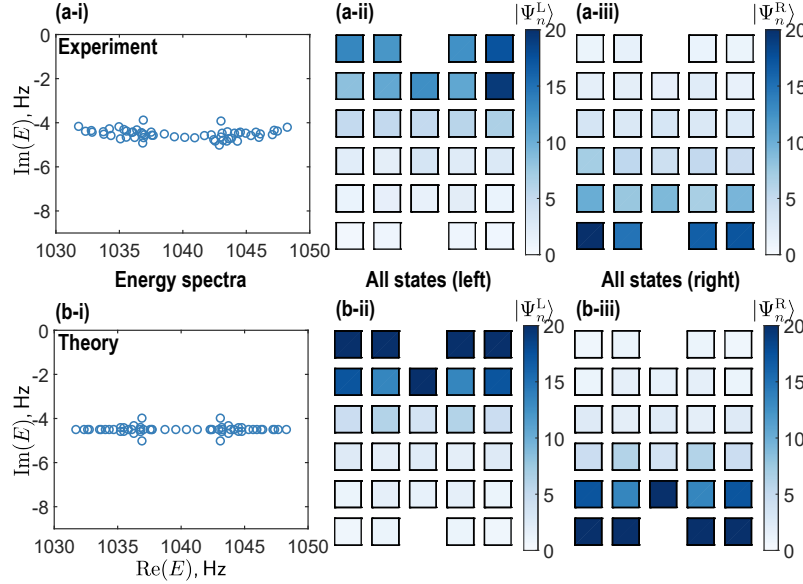

**Figure S28:** (a) Experimental results and (b) theoretical predictions of NH acoustic Chern insulators with an edge dislocation-antidislocation pair under OBCs in the  $\Gamma$  phase. (i) Energy spectra. Summed amplitude distributions of all (ii) left and (iii) right eigenstates. Parameters:  $\omega_0 = 1040\text{ Hz} - 4.5i\text{ Hz}$ ,  $t_0 = m_0 = 3\text{ Hz}$ ,  $h_y = 0.9\text{ Hz}$ ,  $h_x = h_z = 0$ .

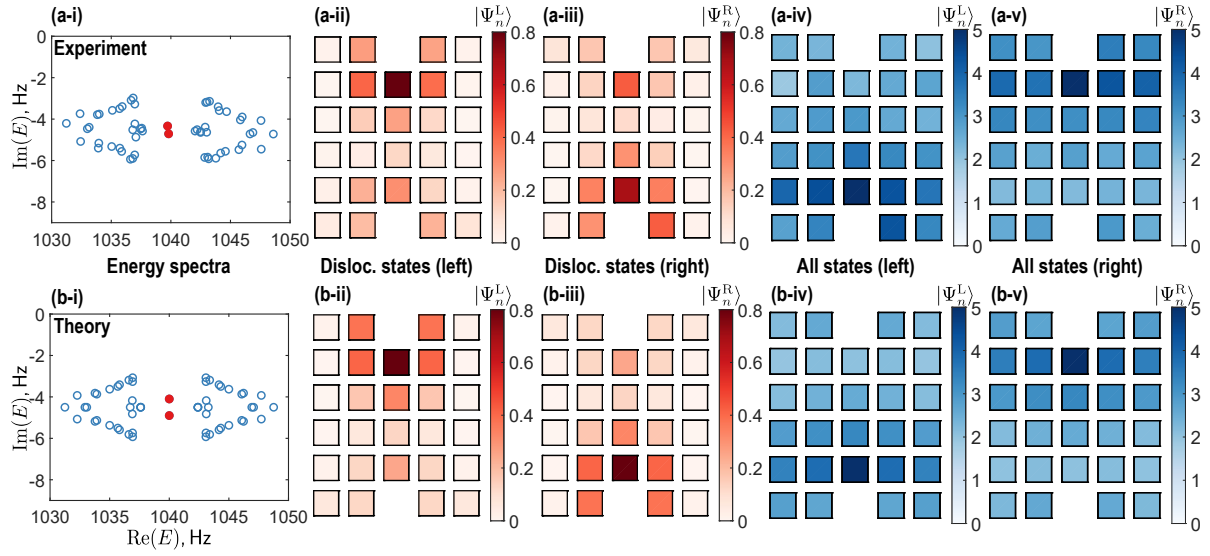

**Figure S29:** (a) Experimental results and (b) theoretical predictions of NH acoustic Chern insulators with an edge dislocation-antidislocation pair under PBCs in the M phase. (i) Energy spectra. Red dots ●, dislocation states; Blue circles ○, other states. Amplitude distributions of the (ii) left and (iii) right eigenstates for the NHDSs. Summed amplitude distributions of all (iv) left and (v) right eigenstates. Parameters:  $\omega_0 = 1040 \text{ Hz} - 4.5i \text{ Hz}$ ,  $t_0 = -m_0 = 3 \text{ Hz}$ ,  $h_y = 1.8 \text{ Hz}$ ,  $h_x = h_z = 0$ .

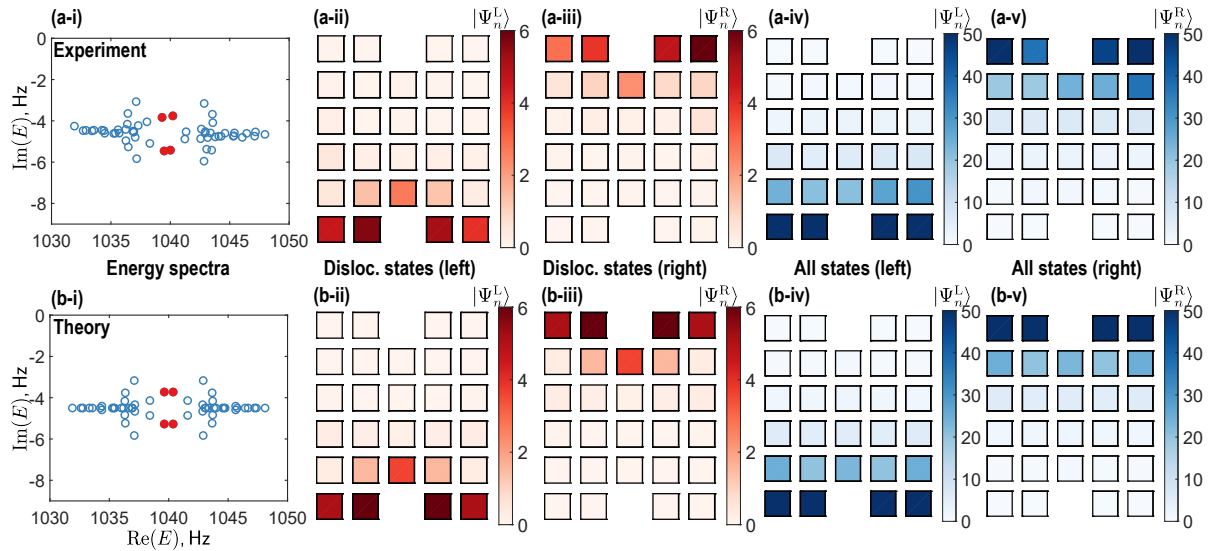

**Figure S30:** (a) Experimental results and (b) theoretical predictions of NH acoustic Chern insulators with an edge dislocation-antidislocation pair under OBCs in the M phase. (i) Energy spectra. Red dots ●, dislocation states; Blue circles ○, other states. Summed amplitude distributions of the (ii) left and (iii) right eigenstates for the NHDS. Summed amplitude distributions of all (iv) left and (v) right eigenstates. Parameters:  $\omega_0 = 1040 \text{ Hz} - 4.5i \text{ Hz}$ ,  $t_0 = -m_0 = 3 \text{ Hz}$ ,  $h_y = 1.8 \text{ Hz}$ ,  $h_x = h_z = 0$ .

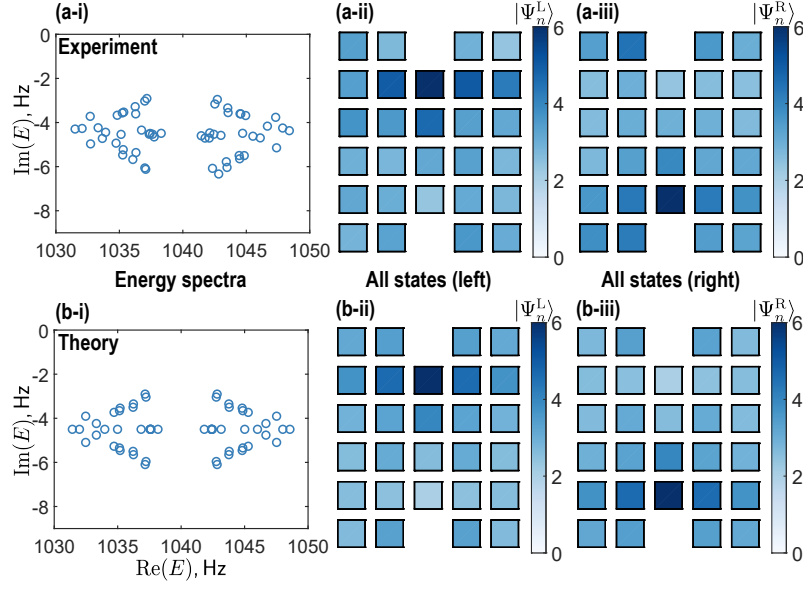

**Figure S31:** (a) Experimental results and (b) theoretical predictions of NH acoustic Chern insulators with an edge dislocation-antidislocation pair under PBCs in the  $\Gamma$  phase. (i) Energy spectra. Summed amplitude distributions of all (ii) left and (iii) right eigenstates. Parameters:  $\omega_0 = 1040\text{Hz} - 4.5i\text{Hz}$ ,  $t_0 = m_0 = 3\text{Hz}$ ,  $h_y = 1.8\text{Hz}$ ,  $h_x = h_z = 0$ .

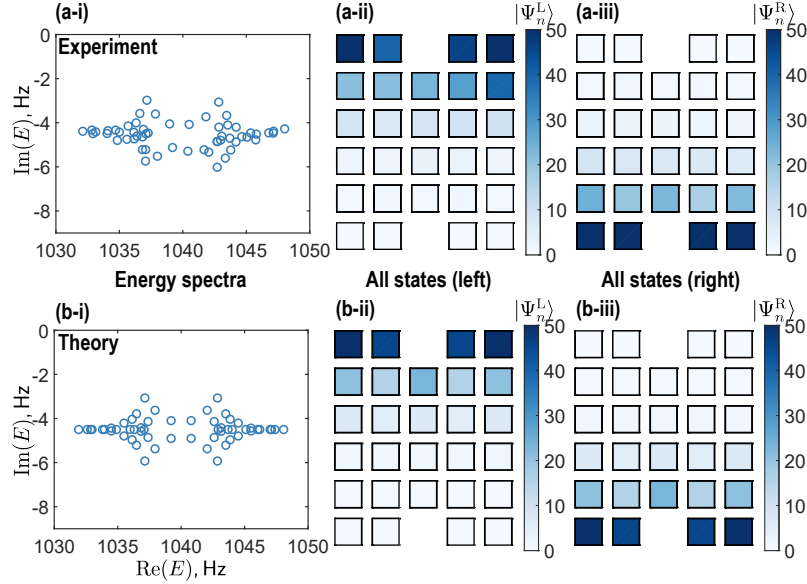

**Figure S32:** (a) Experimental results and (b) theoretical predictions of NH acoustic Chern insulators with an edge dislocation-antidislocation pair under OBCs in the  $\Gamma$  phase. (i) Energy spectra. Summed amplitude distributions of all (ii) left and (iii) right eigenstates. Parameters:  $\omega_0 = 1040\text{Hz} - 4.5i\text{Hz}$ ,  $t_0 = m_0 = 3\text{Hz}$ ,  $h_y = 1.8\text{Hz}$ ,  $h_x = h_z = 0$ .

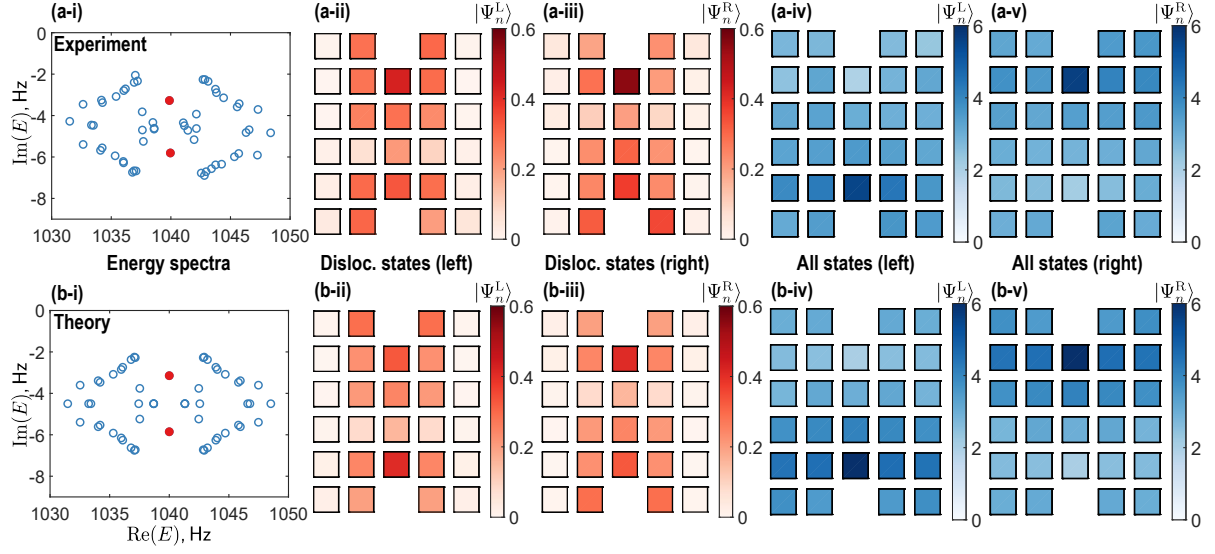

**Figure S33:** (a) Experimental results and (b) theoretical predictions of NH acoustic Chern insulators with an edge dislocation-antidislocation pair under PBCs in the M phase. (i) Energy spectra. Red dots •, dislocation states; Blue circles ○, other states. Amplitude distributions of the (ii) left and (iii) right eigenstates for the NHDS. Summed amplitude distributions of all (iv) left and (v) right eigenstates. Parameters:  $\omega_0 = 1040 \text{ Hz} - 4.5i \text{ Hz}$ ,  $t_0 = -m_0 = 3 \text{ Hz}$ ,  $h_y = 2.7 \text{ Hz}$ ,  $h_x = h_z = 0$ .

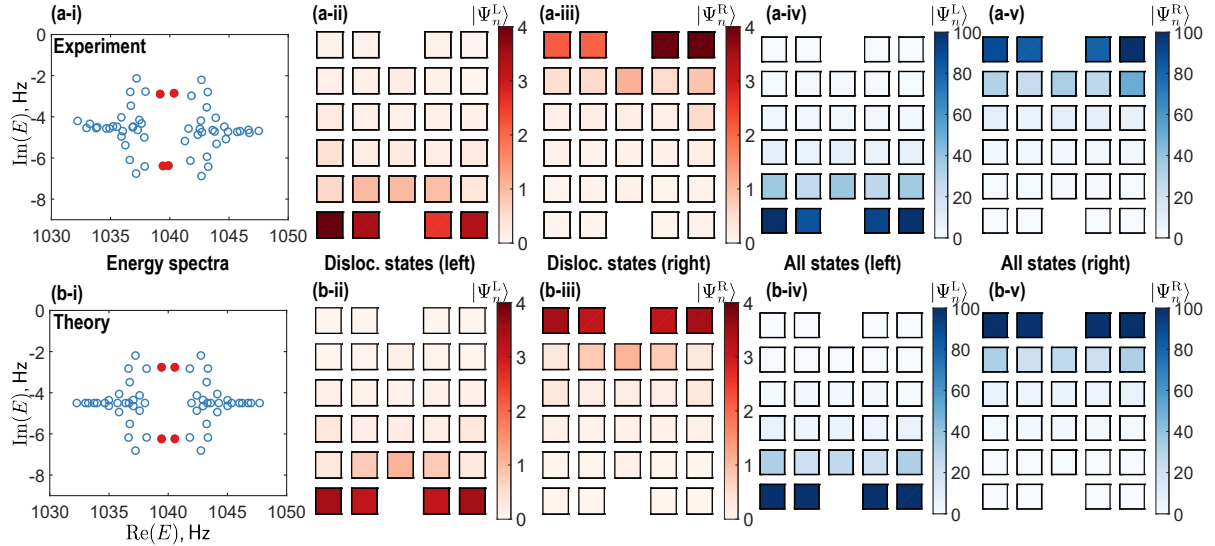

**Figure S34:** (a) Experimental results and (b) theoretical predictions of NH acoustic Chern insulators with an edge dislocation-antidislocation pair under OBCs in the M phase. (i) Energy spectra. Red dots •, dislocation states; Blue circles ○, other states. Summed amplitude distributions of the (ii) left and (iii) right eigenstates for NHDS. Summed amplitude distributions of all (iv) left and (v) right eigenstates. Parameters:  $\omega_0 = 1040 \text{ Hz} - 4.5i \text{ Hz}$ ,  $t_0 = -m_0 = 3 \text{ Hz}$ ,  $h_x = 2.7 \text{ Hz}$ ,  $h_y = h_z = 0$ .

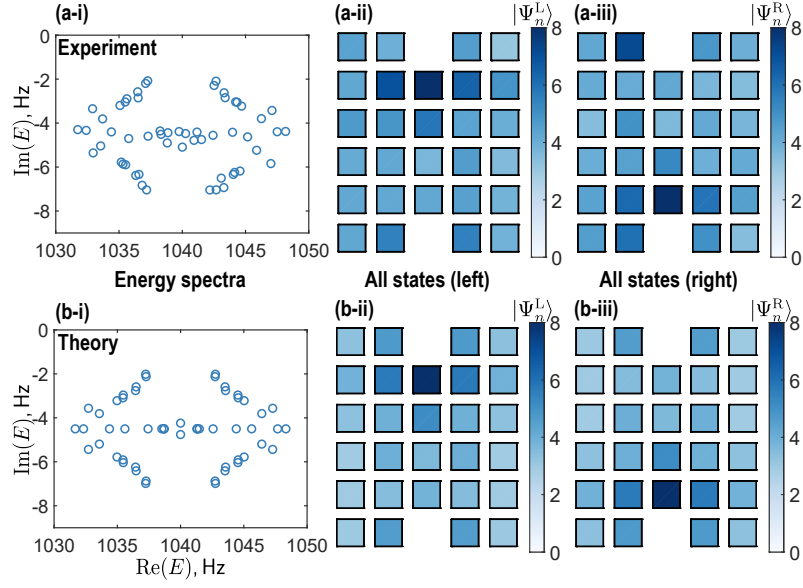

**Figure S35:** (a) Experimental results and (b) theoretical predictions of NH acoustic Chern insulators with an edge dislocation-antidislocation pair under PBCs in the  $\Gamma$  phase. (i) Energy spectra. Summed amplitude distributions of all (ii) left and (iii) right eigenstates. Parameters:  $\omega_0 = 1040\text{Hz} - 4.5i\text{Hz}$ ,  $t_0 = m_0 = 3\text{Hz}$ ,  $h_y = 2.7\text{Hz}$ ,  $h_x = h_z = 0$ .

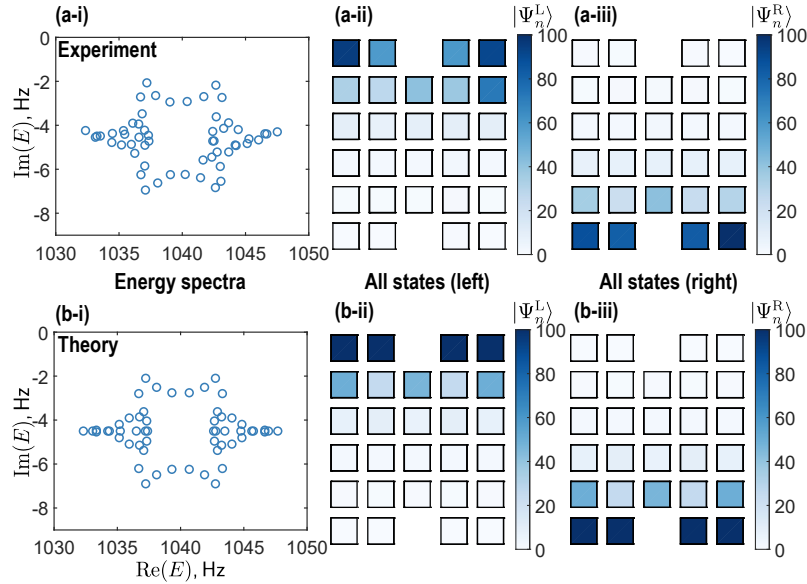

**Figure S36:** (a) Experimental results and (b) theoretical predictions of NH acoustic Chern insulators with an edge dislocation-antidislocation pair under OBCs in the  $\Gamma$  phase. (i) Energy spectra. Summed amplitude distributions of all (ii) left and (iii) right eigenstates. Parameters:  $\omega_0 = 1040\text{Hz} - 4.5i\text{Hz}$ ,  $t_0 = m_0 = 3\text{Hz}$ ,  $h_x = 2.7\text{Hz}$ ,  $h_y = h_z = 0$ .

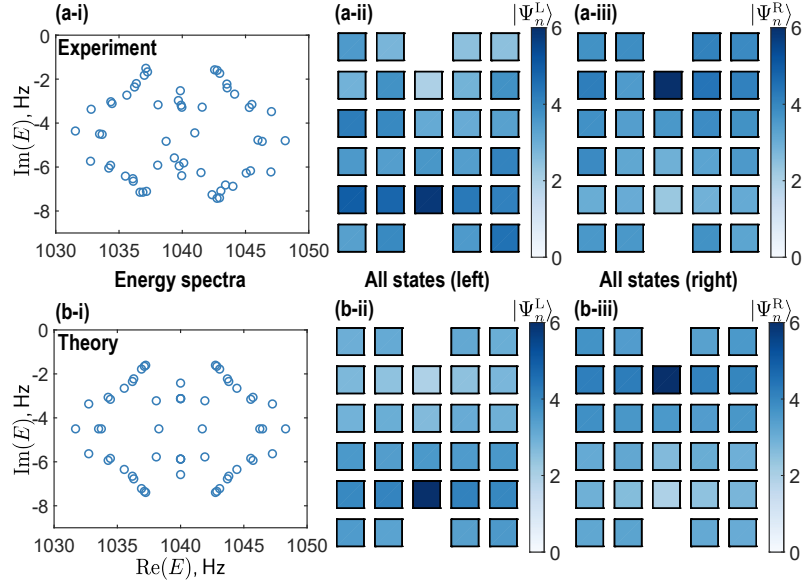

**Figure S37:** (a) Experimental results and (b) theoretical predictions of NH acoustic Chern insulators with an edge dislocation-antidislocation pair under PBCs in the M phase. (i) Energy spectra. Summed amplitude distributions of all (ii) left and (iii) right eigenstates. Parameters:  $\omega_0 = 1040\text{Hz} - 4.5i\text{Hz}$ ,  $t_0 = -m_0 = 3\text{Hz}$ ,  $h_y = 3.3\text{Hz}$ ,  $h_x = h_z = 0$ .

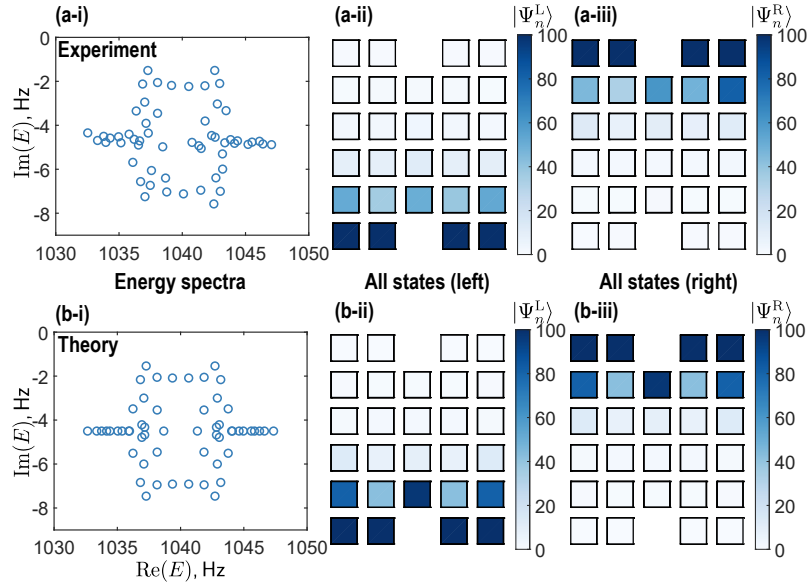

**Figure S38:** (a) Experimental results and (b) theoretical predictions of NH acoustic Chern insulators with an edge dislocation-antidislocation pair under OBCs in the M phase. (i) Energy spectra. Summed amplitude distributions of all (ii) left and (iii) right eigenstates. Parameters:  $\omega_0 = 1040\text{Hz} - 4.5i\text{Hz}$ ,  $t_0 = -m_0 = 3\text{Hz}$ ,  $h_x = 3.3\text{Hz}$ ,  $h_y = h_z = 0$ .

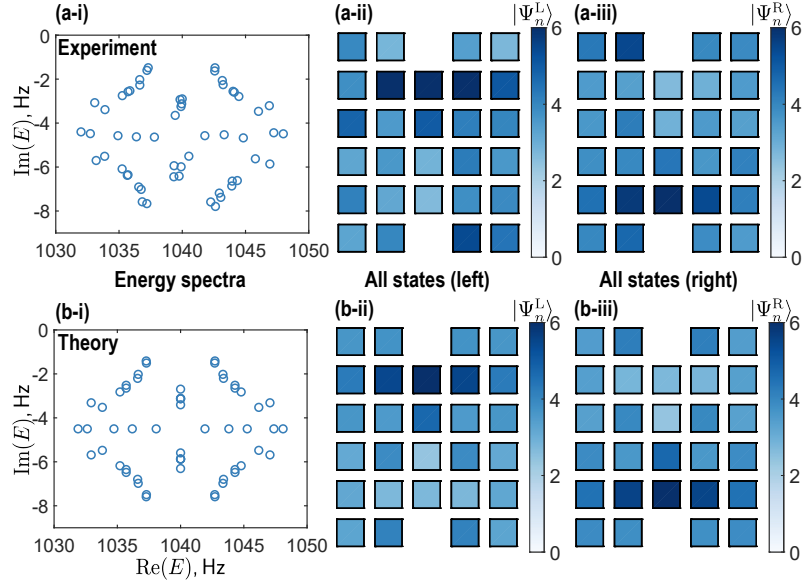

**Figure S39:** (a) Experimental results and (b) theoretical predictions of NH acoustic Chern insulators with an edge dislocation-antidislocation pair under PBCs in the  $\Gamma$  phase. (i) Energy spectra. Summed amplitude distributions of all (ii) left and (iii) right eigenstates. Parameters:  $\omega_0 = 1040\text{Hz} - 4.5i\text{Hz}$ ,  $t_0 = m_0 = 3\text{Hz}$ ,  $h_y = 3.3\text{Hz}$ ,  $h_x = h_z = 0$ .

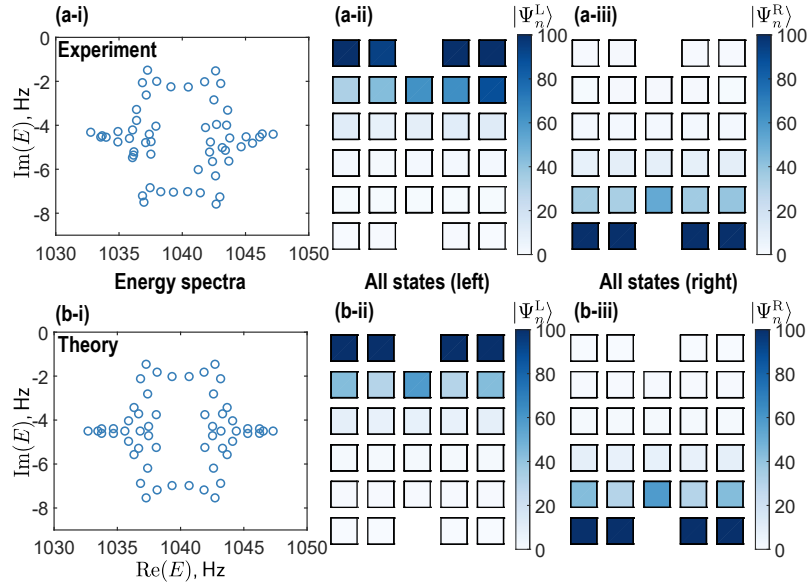

**Figure S40:** (a) Experimental results and (b) theoretical predictions of NH acoustic Chern insulators with an edge dislocation-antidislocation pair under OBCs in the  $\Gamma$  phase. (i) Energy spectra. (ii–iii) Summed amplitude distributions of all (ii) left and (iii) right eigenstates. Parameters:  $\omega_0 = 1040\text{Hz} - 4.5i\text{Hz}$ ,  $t_0 = m_0 = 3\text{Hz}$ ,  $h_x = 3.3\text{Hz}$ ,  $h_y = h_z = 0$ .

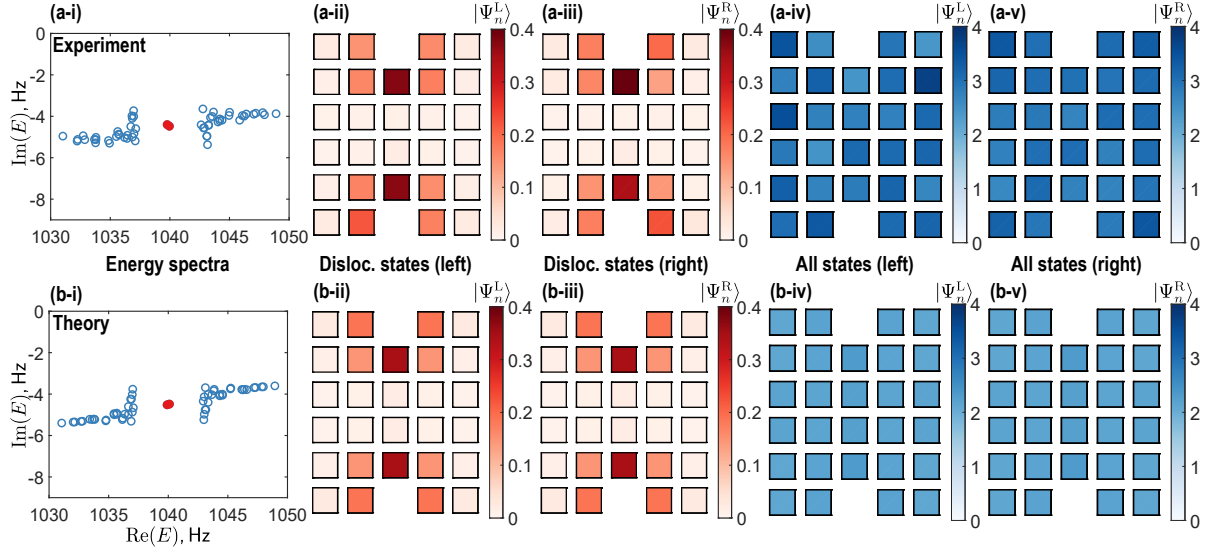

**Figure S41:** (a) Experimental results and (b) theoretical predictions of NH acoustic Chern insulators with an edge dislocation-antidislocation pair under PBCs in the M phase. (i) Energy spectra. Red dots •, dislocation states; Blue circles ○, other states. Amplitude distributions of the (ii) left and (iii) right eigenstates for the dislocation states. Summed amplitude distributions of all (iv) left and (v) right eigenstates. Parameters:  $\omega_0 = 1040 \text{ Hz} - 4.5i \text{ Hz}$ ,  $t_0 = -m_0 = 3 \text{ Hz}$ ,  $h_z = 0.3 \text{ Hz}$ ,  $h_x = h_y = 0$ .

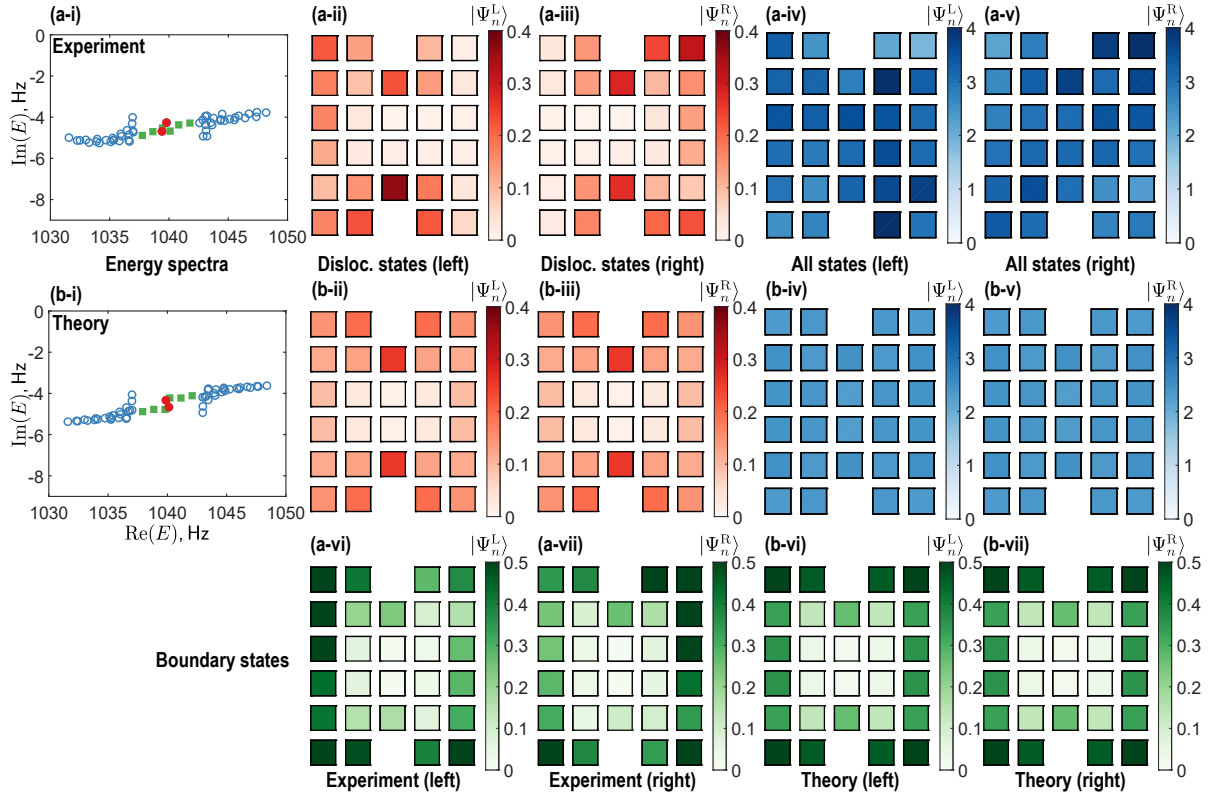

**Figure S42:** (a) Experimental results and (b) theoretical predictions of NH acoustic Chern insulators with an edge dislocation-antidislocation pair under OBCs in the M phase. (i) Energy spectra. Red dots •, dislocation states; green squares ■, boundary states; blue circles ○, all other states. Amplitude distributions of the (ii) left and (iii) right eigenstates for the dislocation states. Summed amplitude distributions of all (iv) left and (v) right eigenstates. Amplitude distributions of the (vi) left and (vii) right eigenstates for the boundary states. Parameters:  $\omega_0 = 1040 \text{ Hz} - 4.5i \text{ Hz}$ ,  $t_0 = -m_0 = 3 \text{ Hz}$ ,  $h_z = 0.3 \text{ Hz}$ ,  $h_x = h_y = 0$ .

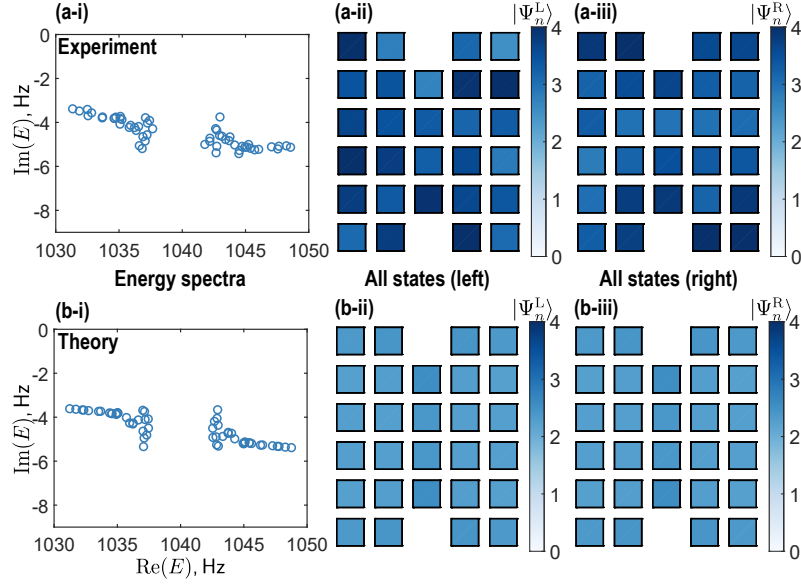

**Figure S43:** (a) Experimental results and (b) theoretical predictions of NH acoustic Chern insulators with an edge dislocation-antidislocation pair under PBCs in the  $\Gamma$  phase. (i) Energy spectra. Summed amplitude distributions of all (ii) left and (iii) right eigenstates. Parameters:  $\omega_0 = 1040\text{Hz} - 4.5i\text{Hz}$ ,  $t_0 = m_0 = 3\text{Hz}$ ,  $h_z = 0.9\text{Hz}$ ,  $h_x = h_y = 0$ .

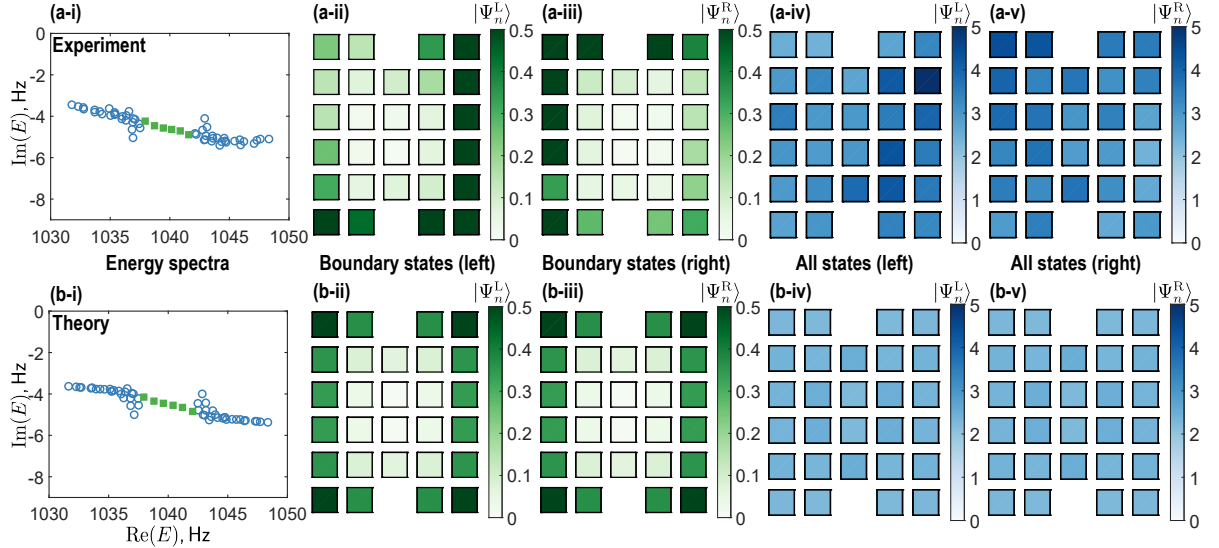

**Figure S44:** (a) Experimental results and (b) theoretical predictions of NH acoustic Chern insulators with an edge dislocation-antidislocation pair under OBCs in the  $\Gamma$  phase. (i) Energy spectra. Green squares ■, boundary states; Blue circles ○, other states. Amplitude distributions of the (ii) left and (iii) right eigenstates for the boundary states. Summed amplitude distributions of all (iv) left and (v) right eigenstates. Parameters:  $\omega_0 = 1040\text{Hz} - 4.5i\text{Hz}$ ,  $t_0 = m_0 = 3\text{Hz}$ ,  $h_z = 0.3\text{Hz}$ ,  $h_y = h_z = 0$ .

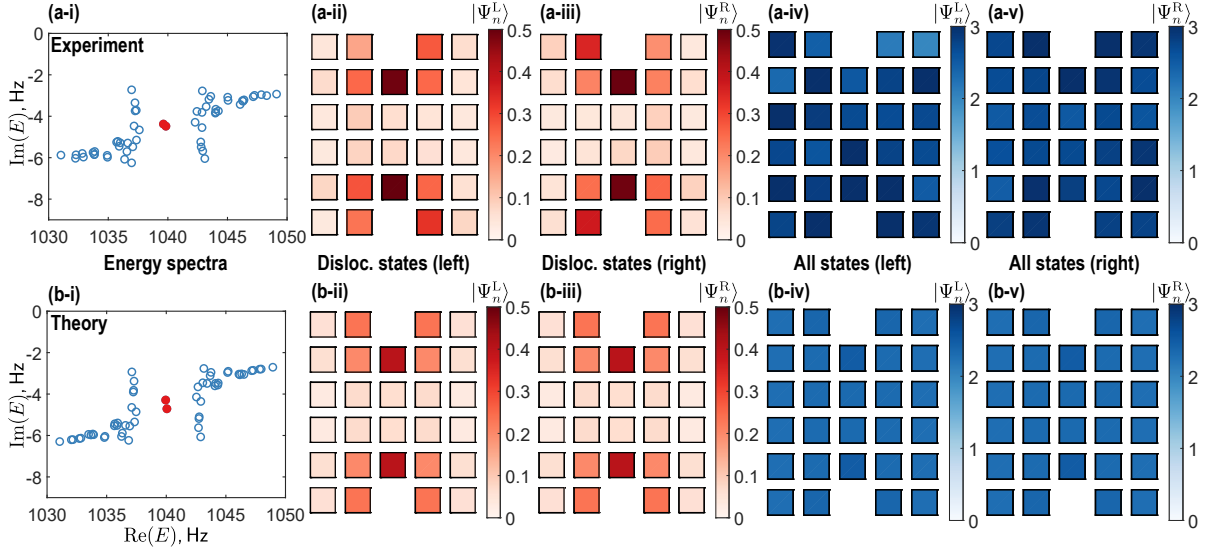

**Figure S45:** (a) Experimental results and (b) theoretical predictions of NH acoustic Chern insulators with an edge dislocation-antidislocation pair under PBCs in the M phase. (i) Energy spectra. Red dots ●, dislocation states; Blue circles ○, other states. Amplitude distributions of the (ii) left and (iii) right eigenstates for the dislocation states. Summed amplitude distributions of all (iv) left and (v) right eigenstates. Parameters:  $\omega_0 = 1040 \text{ Hz} - 4.5i \text{ Hz}$ ,  $t_0 = -m_0 = 3 \text{ Hz}$ ,  $h_z = 1.8 \text{ Hz}$ ,  $h_x = h_y = 0$ .

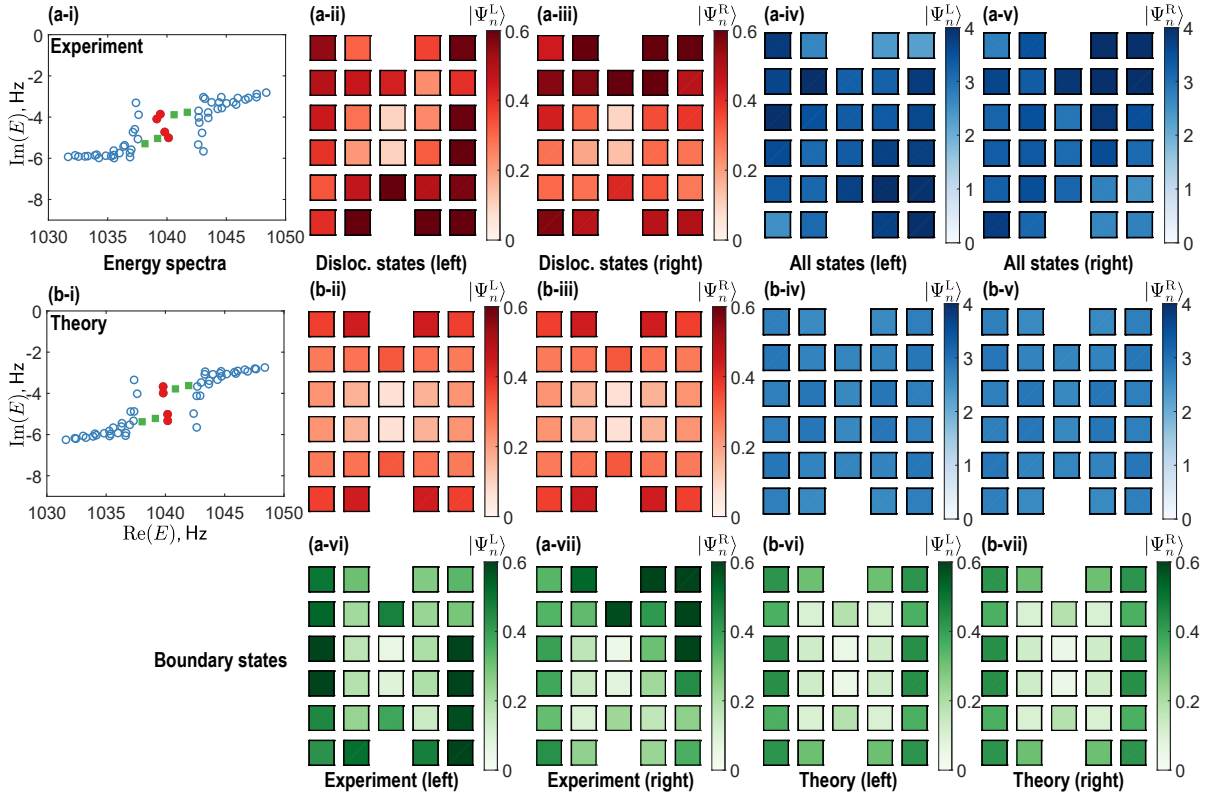

**Figure S46:** (a) Experimental results and (b) theoretical predictions of NH acoustic Chern insulators with an edge dislocation-antidislocation pair under OBCs in the M phase. (i) Energy spectra. Red dots ●, dislocation states; Blue circles ○, other states; Green squares ■, boundary states. Summed amplitude distributions of the (ii) left and (iii) right eigenstates for the dislocation states. Summed amplitude distributions of all (iv) left and (v) right eigenstates. Amplitude distributions of the (vi) left and (vii) right eigenstates for the boundary state. Parameters:  $\omega_0 = 1040 \text{ Hz} - 4.5i \text{ Hz}$ ,  $t_0 = -m_0 = 3 \text{ Hz}$ ,  $h_z = 1.8 \text{ Hz}$ ,  $h_x = h_y = 0$ .

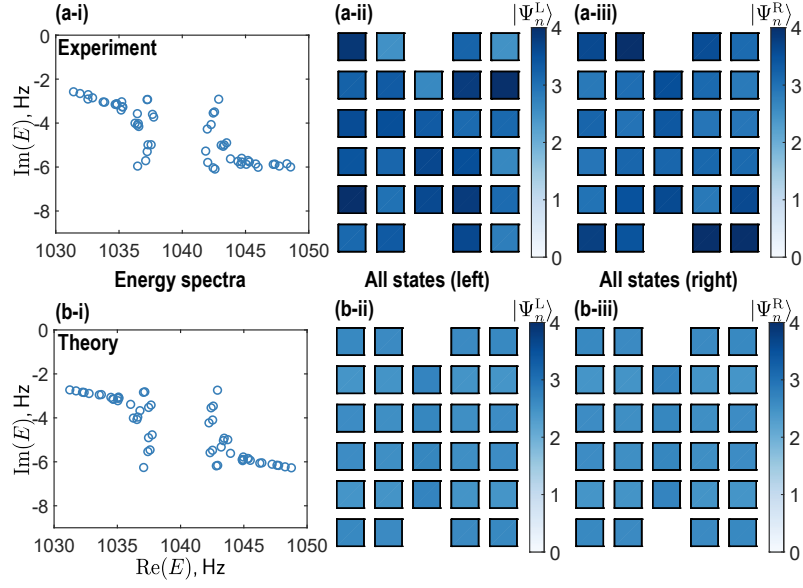

**Figure S47:** (a) Experimental results and (b) theoretical predictions of NH acoustic Chern insulators with an edge dislocation-antidislocation pair under PBCs in the  $\Gamma$  phase. (i) Energy spectra. Summed amplitude distributions of all (ii) left and (iii) right eigenstates. Parameters:  $\omega_0 = 1040\text{Hz} - 4.5i\text{Hz}$ ,  $t_0 = m_0 = 3\text{Hz}$ ,  $h_z = 1.8\text{Hz}$ ,  $h_x = h_y = 0$ .

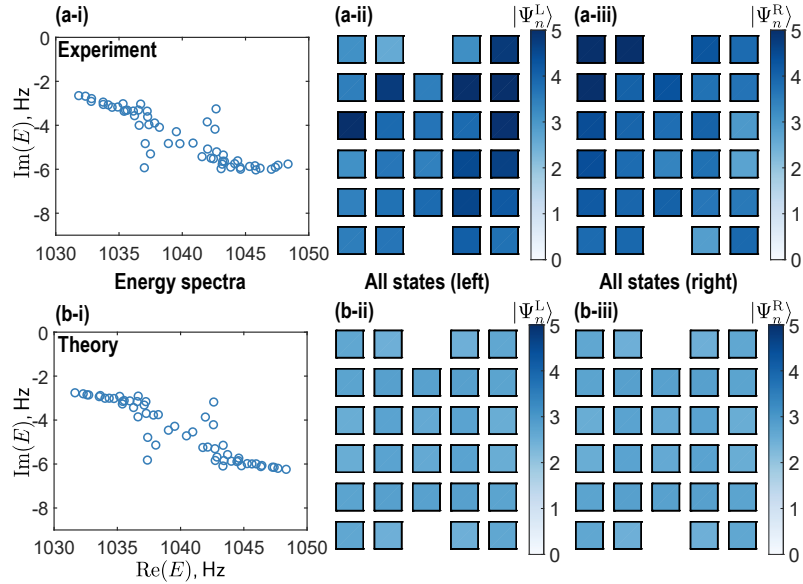

**Figure S48:** (a) Experimental results and (b) theoretical predictions of NH acoustic Chern insulators with an edge dislocation-antidislocation pair under OBCs in the  $\Gamma$  phase. (i) Energy spectra. Summed amplitude distributions of all (ii) left and (iii) right eigenstates. Parameters:  $\omega_0 = 1040\text{Hz} - 4.5i\text{Hz}$ ,  $t_0 = m_0 = 3\text{Hz}$ ,  $h_z = 1.8\text{Hz}$ ,  $h_x = h_y = 0$ .

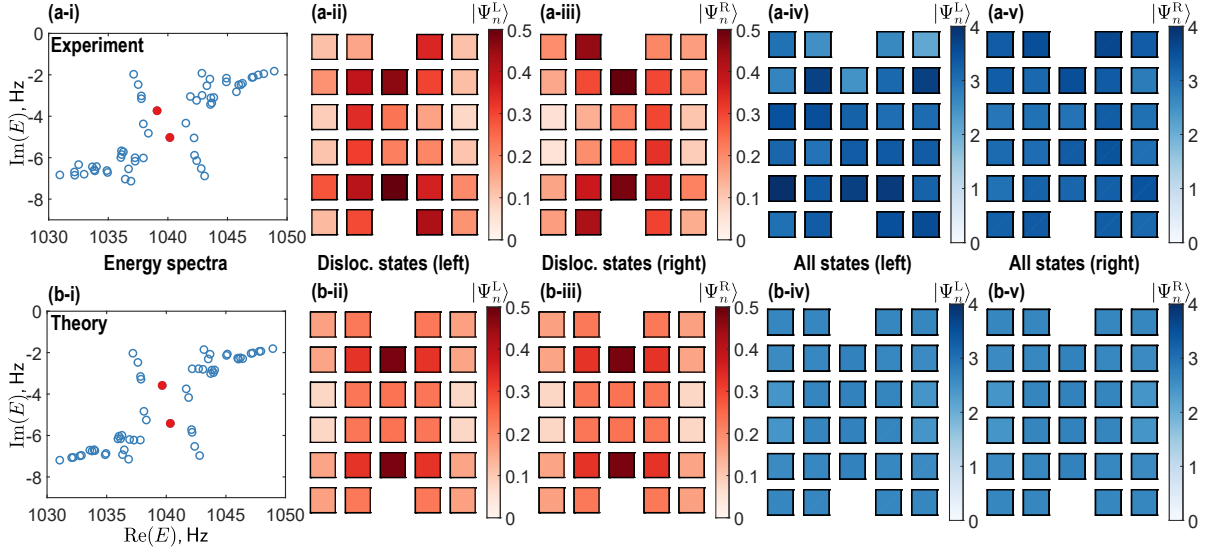

**Figure S49:** (a) Experimental results and (b) theoretical predictions of NH acoustic Chern insulators with an edge dislocation-antidislocation pair under PBCs in the M phase. (i) Energy spectra. Red dots ●, dislocation states; Blue circles ○, other states. Amplitude distributions of the (ii) left and (iii) right eigenstates for the dislocation states. Summed amplitude distributions of all (iv) left and (v) right eigenstates. Parameters:  $\omega_0 = 1040 \text{ Hz} - 4.5i \text{ Hz}$ ,  $t_0 = -m_0 = 3 \text{ Hz}$ ,  $h_z = 2.7 \text{ Hz}$ ,  $h_x = h_y = 0$ .

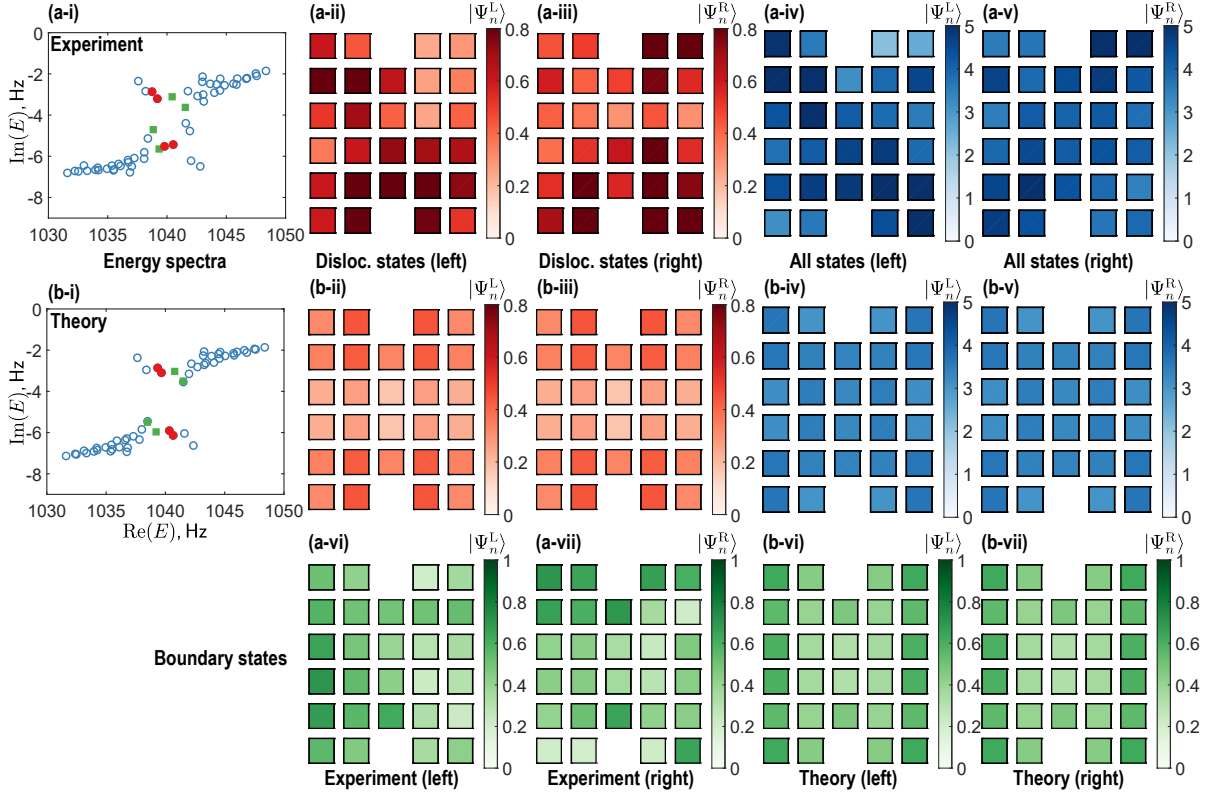

**Figure S50:** (a) Experimental results and (b) theoretical predictions of NH acoustic Chern insulators with an edge dislocation-antidislocation pair under OBCs in the M phase. (i) Energy spectra. Red dots ●, dislocation states; Blue circles ○, other states; Green squares ■, boundary states. Summed amplitude distributions of the (ii) left and (iii) right eigenstates for the dislocation states. Summed amplitude distributions of all (iv) left and (v) right eigenstates. Amplitude distributions of the (vi) left and (vii) right eigenstates for the boundary state. Parameters:  $\omega_0 = 1040 \text{ Hz} - 4.5i \text{ Hz}$ ,  $t_0 = -m_0 = 3 \text{ Hz}$ ,  $h_z = 2.7 \text{ Hz}$ ,  $h_x = h_y = 0$ .

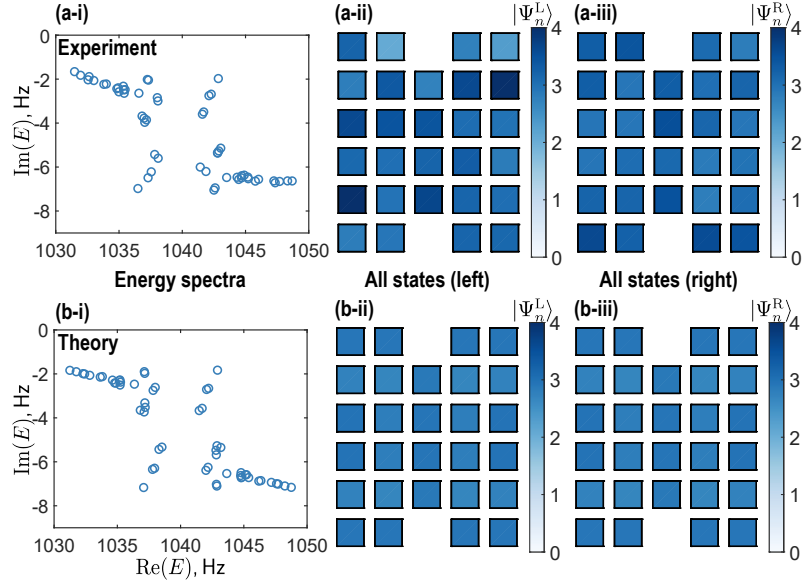

**Figure S51:** (a) Experimental results and (b) theoretical predictions of NH acoustic Chern insulators with an edge dislocation-antidislocation pair under PBCs in the  $\Gamma$  phase. (i) Energy spectra. Summed amplitude distributions of all (ii) left and (iii) right eigenstates. Parameters:  $\omega_0 = 1040\text{Hz} - 4.5i\text{Hz}$ ,  $t_0 = m_0 = 3\text{Hz}$ ,  $h_z = 2.7\text{Hz}$ ,  $h_x = h_y = 0$ .

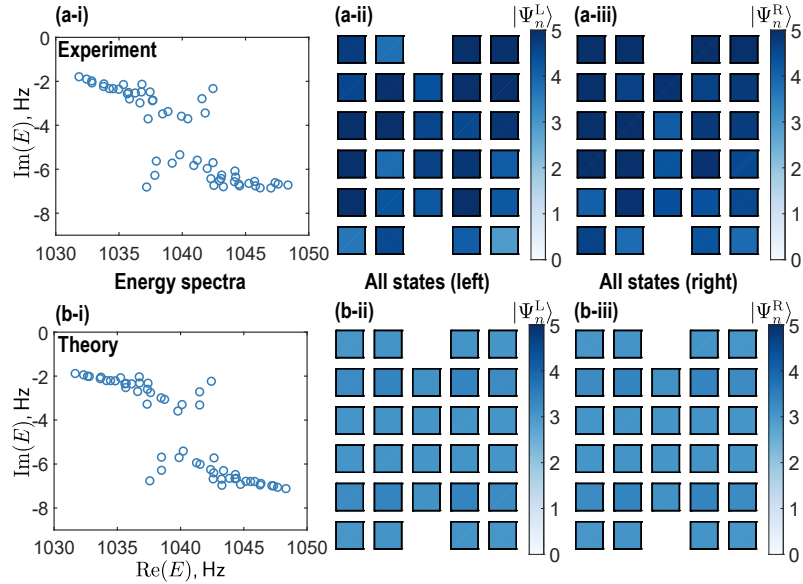

**Figure S52:** (a) Experimental results and (b) theoretical predictions of NH acoustic Chern insulators with an edge dislocation-antidislocation pair under OBCs in the  $\Gamma$  phase. (i) Energy spectra. Summed amplitude distributions of all (ii) left and (iii) right eigenstates. Parameters:  $\omega_0 = 1040\text{Hz} - 4.5i\text{Hz}$ ,  $t_0 = m_0 = 3\text{Hz}$ ,  $h_z = 2.7\text{Hz}$ ,  $h_x = h_y = 0$ .

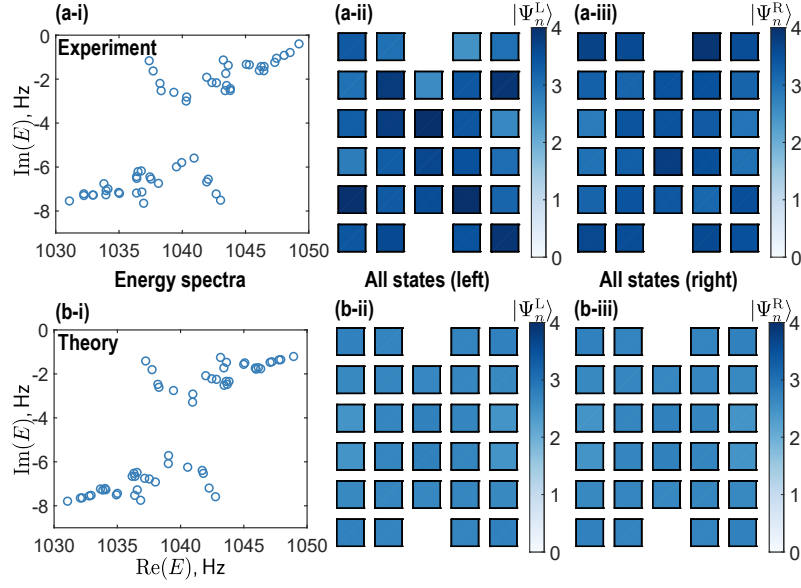

**Figure S53:** (a) Experimental results and (b) theoretical predictions of NH acoustic Chern insulators with an edge dislocation-antidislocation pair under OBCs in the M phase. (i) Energy spectra. Summed amplitude distributions of all (ii) left and (iii) right eigenstates. Parameters:  $\omega_0 = 1040\text{Hz} - 4.5i\text{Hz}$ ,  $t_0 = -m_0 = 3\text{Hz}$ ,  $h_z = 3.3\text{Hz}$ ,  $h_x = h_y = 0$ .

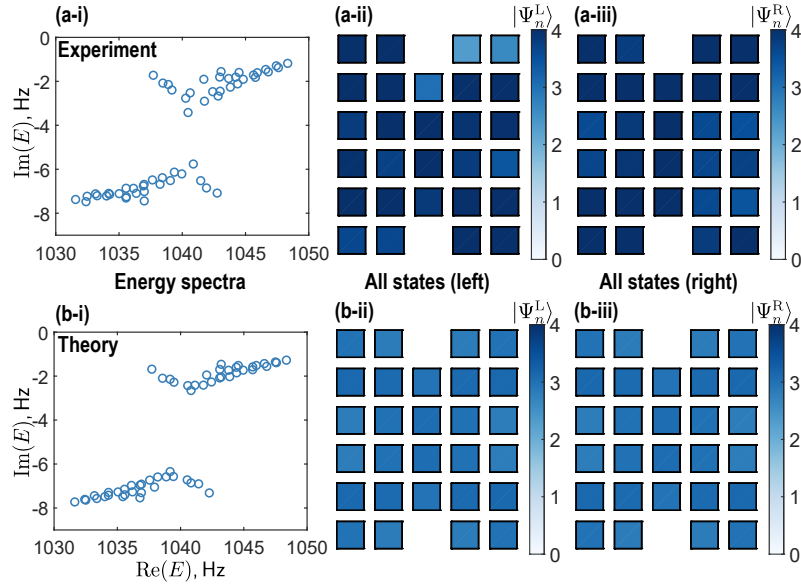

**Figure S54:** (a) Experimental results and (b) theoretical predictions of NH acoustic Chern insulators with an edge dislocation-antidislocation pair under OBCs in the M phase. (i) Energy spectra. Summed amplitude distributions of all (ii) left and (iii) right eigenstates. Parameters:  $\omega_0 = 1040\text{Hz} - 4.5i\text{Hz}$ ,  $t_0 = -m_0 = 3\text{Hz}$ ,  $h_z = 3.3\text{Hz}$ ,  $h_x = h_y = 0$ .

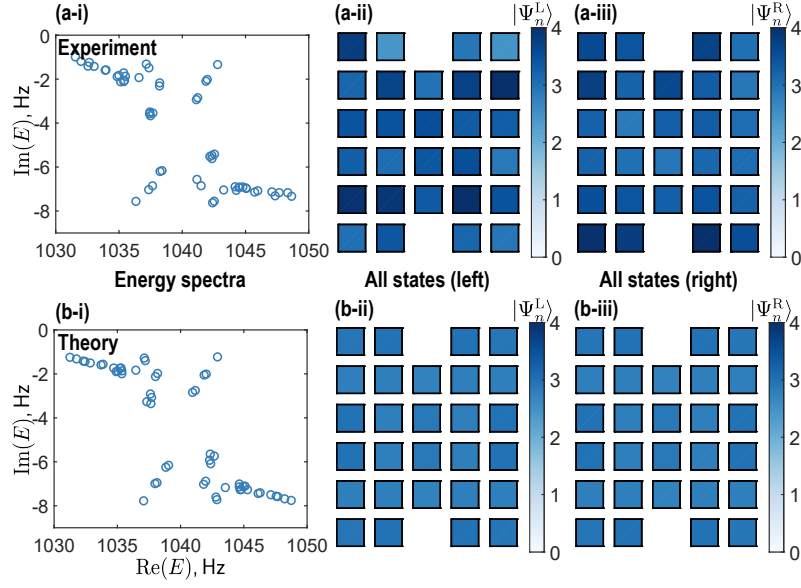

**Figure S55:** (a) Experimental results and (b) theoretical predictions of NH acoustic Chern insulators with an edge dislocation-antidislocation pair under PBCs in the  $\Gamma$  phase. (i) Energy spectra. Summed amplitude distributions of all (ii) left and (iii) right eigenstates. Parameters:  $\omega_0 = 1040\text{Hz} - 4.5i\text{Hz}$ ,  $t_0 = m_0 = 3\text{Hz}$ ,  $h_z = 3.3\text{Hz}$ ,  $h_x = h_y = 0$ .

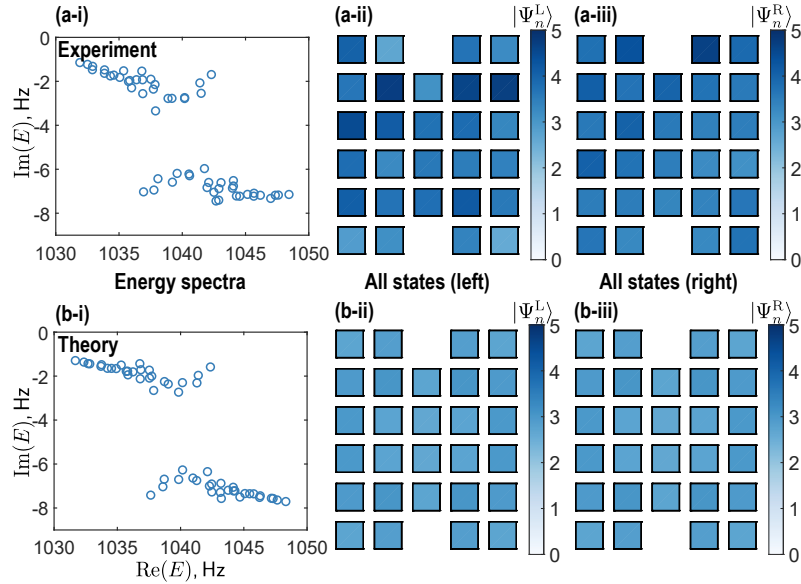

**Figure S56:** (a) Experimental results and (b) theoretical predictions of NH acoustic Chern insulators with an edge dislocation-antidislocation pair under OBCs in the  $\Gamma$  phase. (i) Energy spectra. Summed amplitude distributions of all (ii) left and (iii) right eigenstates. Parameters:  $\omega_0 = 1040\text{Hz} - 4.5i\text{Hz}$ ,  $t_0 = m_0 = 3\text{Hz}$ ,  $h_z = 3.3\text{Hz}$ ,  $h_x = h_y = 0$ .

## References

- [1] J.-X. Zhong et al. *Experimentally Probing Non-Hermitian Spectral Transition and Eigenstate Skewness*. 2025. URL: <http://arxiv.org/abs/2501.08160> (visited on 02/19/2025). Pre-published.
